# Supplementary material for: Examination of the adiabatic approximation for $(d,p)$ reactions
Source: arXiv:1702.03135 ancillary file (2017-06-15)

## Addendum to “Examination of the adiabatic approximation for $(d, p)$ reactions”

Yoshiki Chazono,<sup>1,\*</sup> Kazuki Yoshida,<sup>1</sup> and Kazuyuki Ogata<sup>1</sup>

<sup>1</sup>*Research Center for Nuclear Physics (RCNP), Osaka University, Ibaraki 567-0047, Japan*

(Dated: March 24, 2017)

In the following we display the angular distribution of the  $A(d, p)B$  cross sections for the 128 reaction systems discussed in the article. Each page corresponds to a specific choice of the target nucleus  $A$ , transferred angular momentum  $\ell_f$ , and neutron separation energy  $S_n$ . On the left side, comparison between CDCC (solid line) and CDCC-BA (dashed line) is shown, whereas on the right side the result of CDCC (solid line) is compared with that ignoring the closed channels (dashed line). Results at 5, 10, 20, and 40 MeV are shown in the top, middle-upper, middle-lower, and bottom panels, respectively. On top of each panel, information on the reaction system is given.

---

\*chazono@rcnp.osaka-u.ac.jp

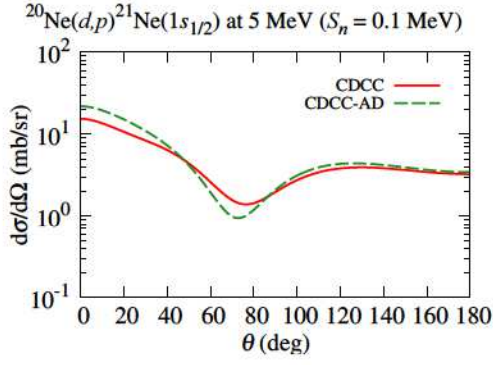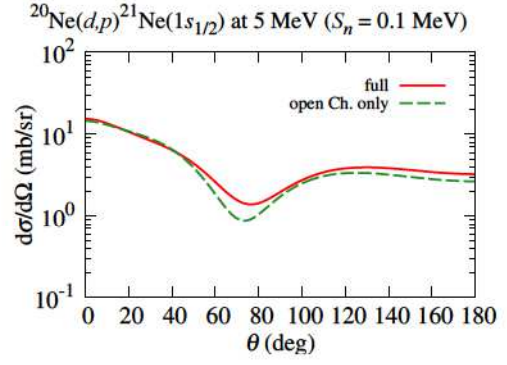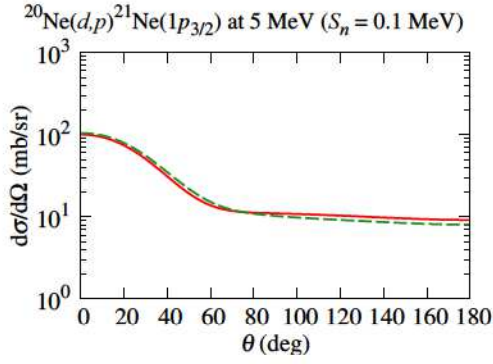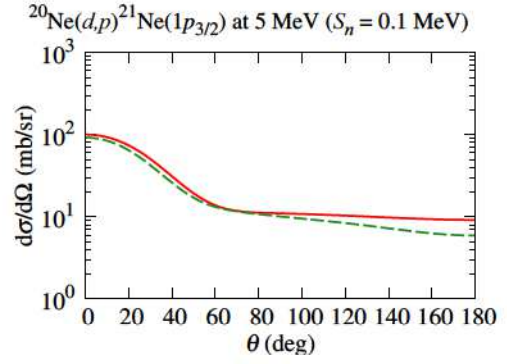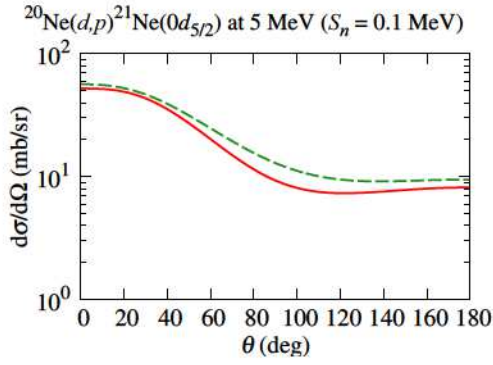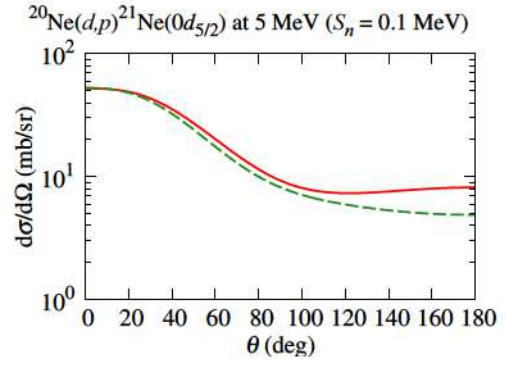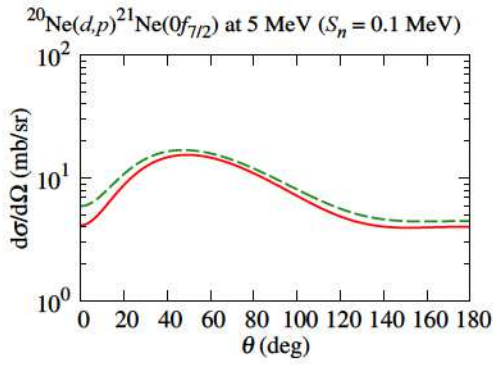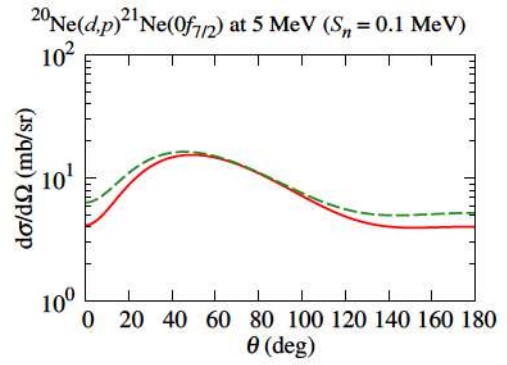

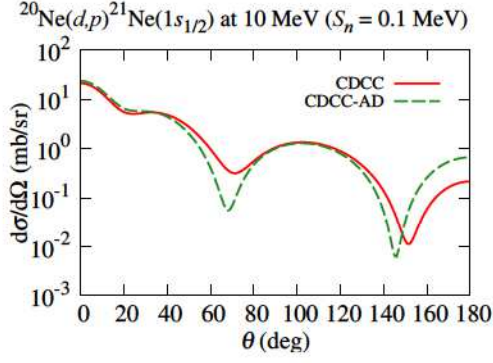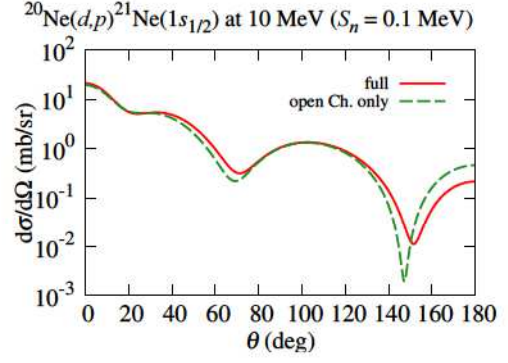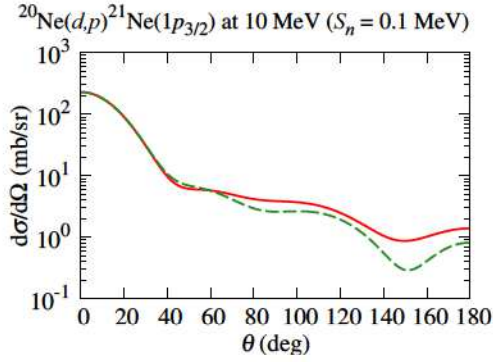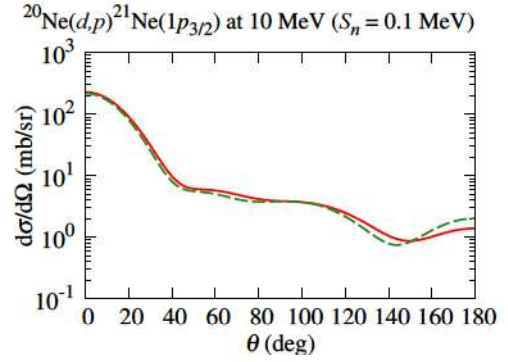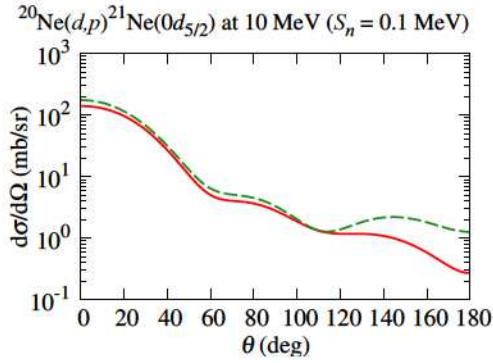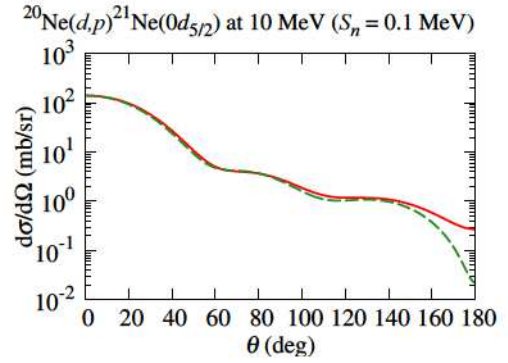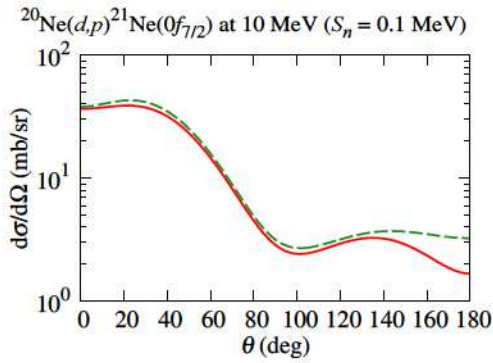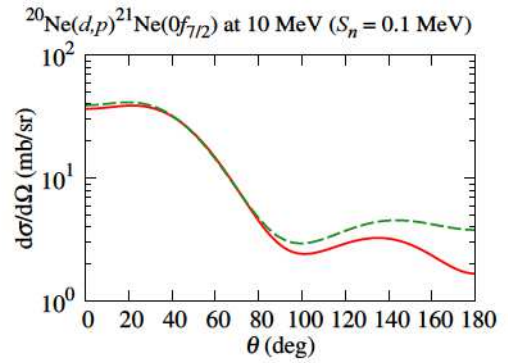

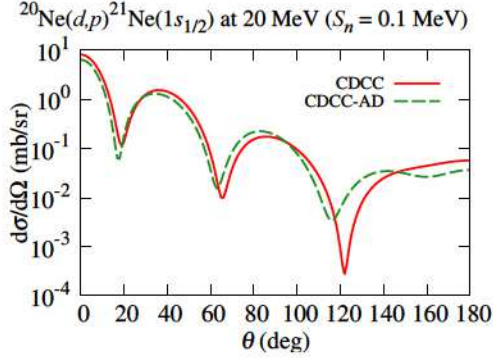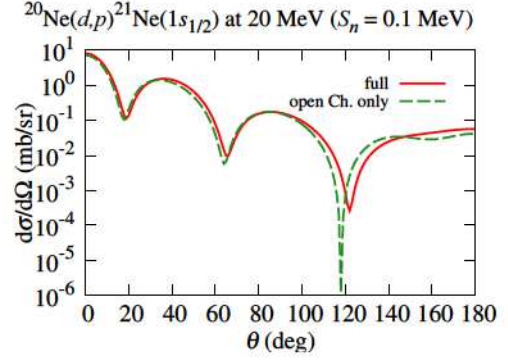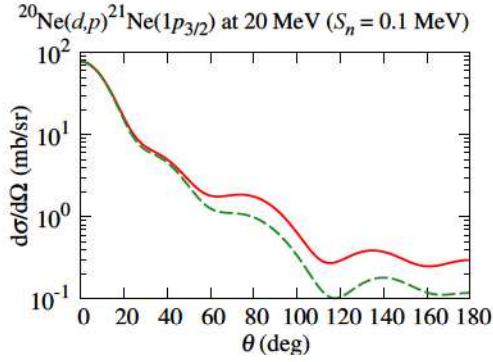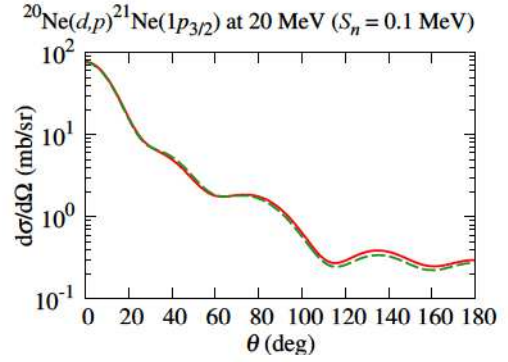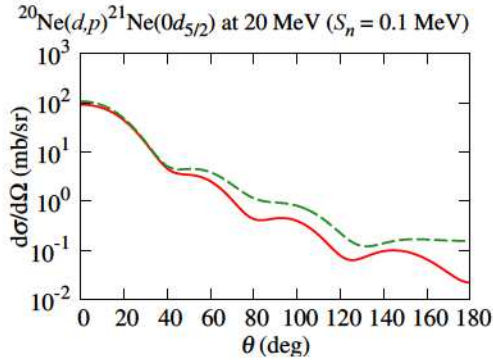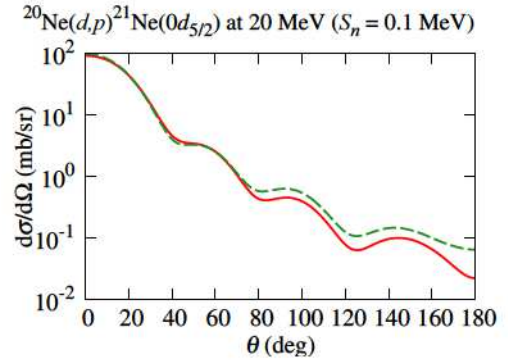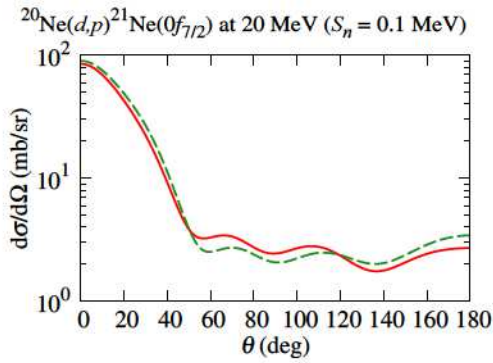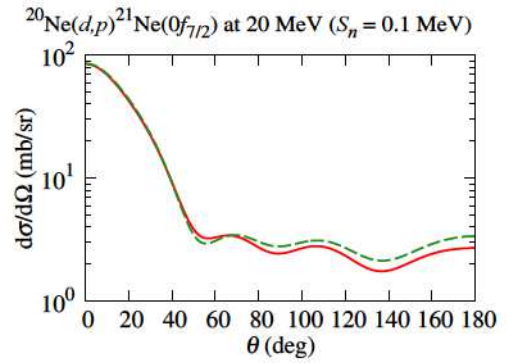



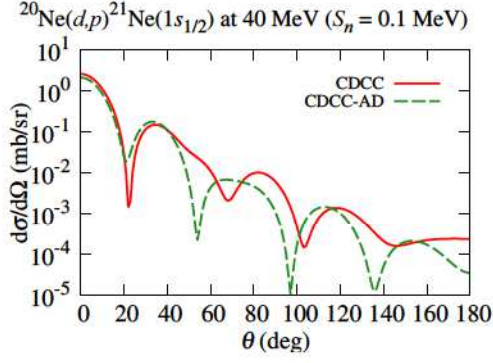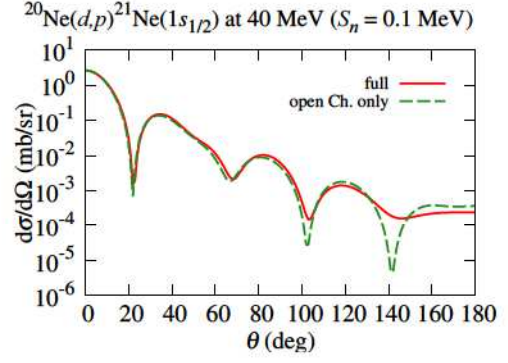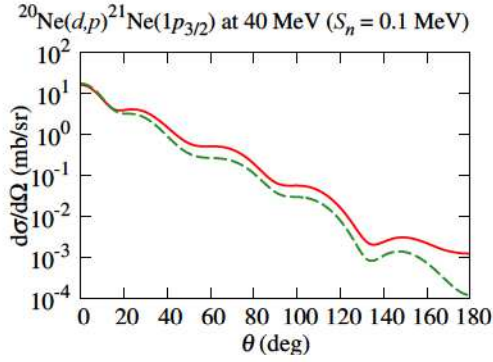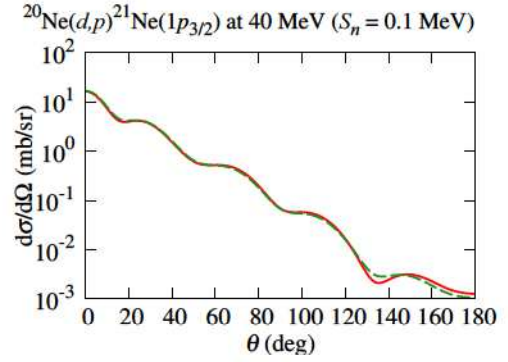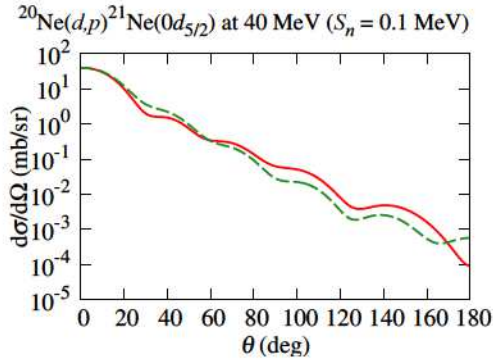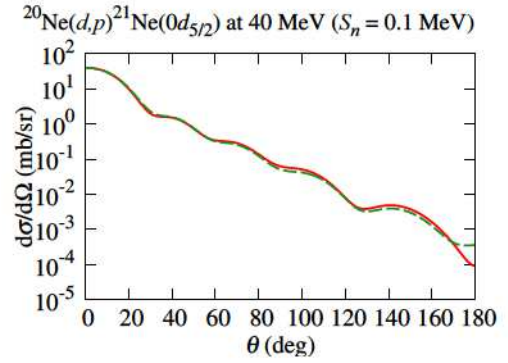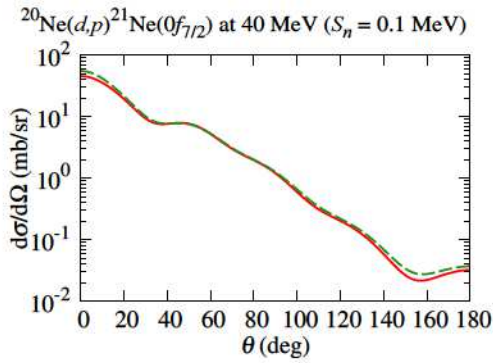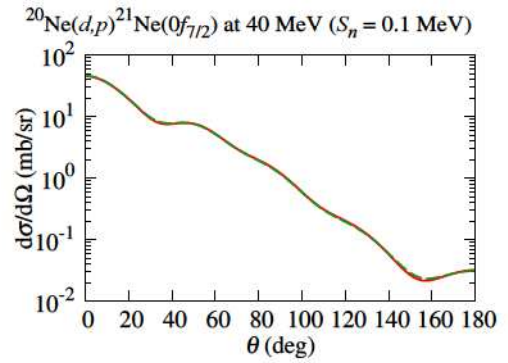

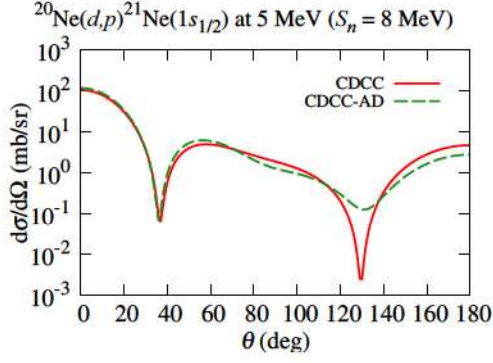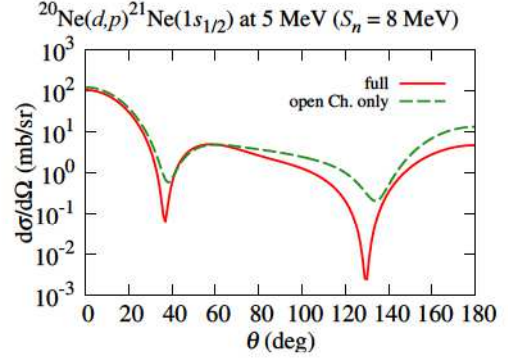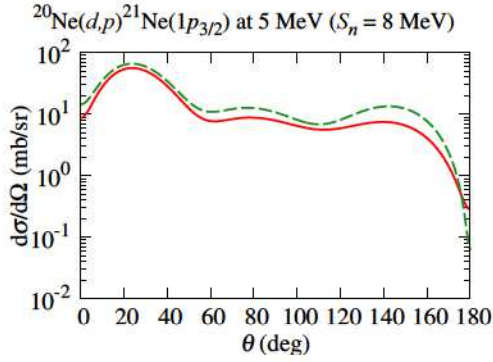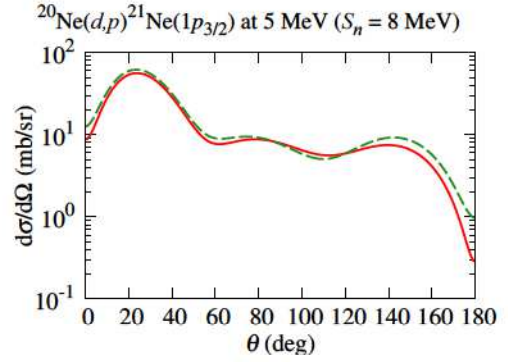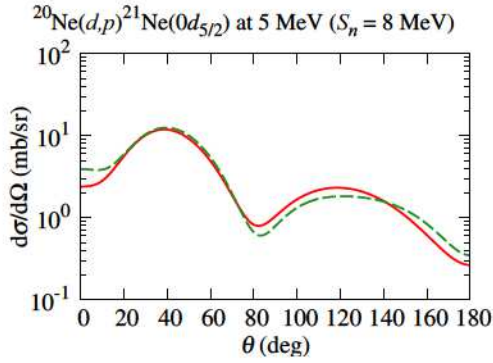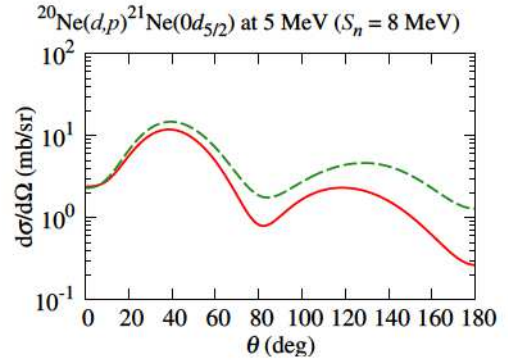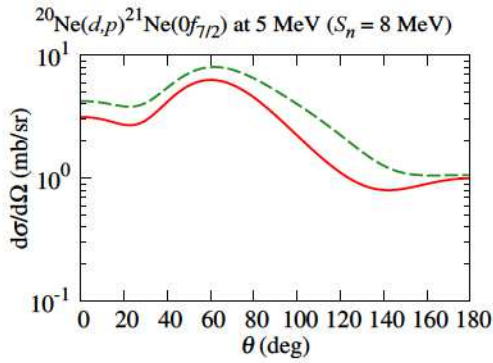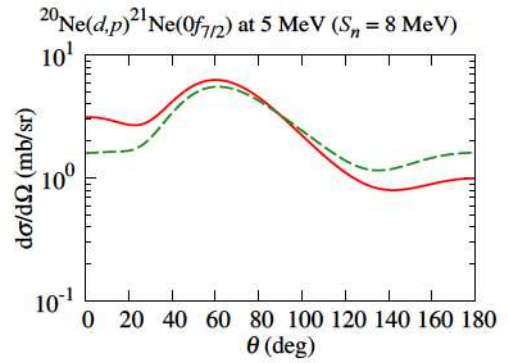

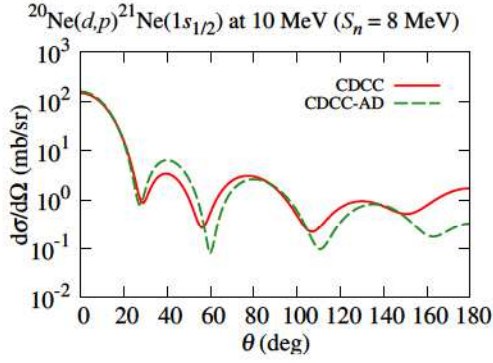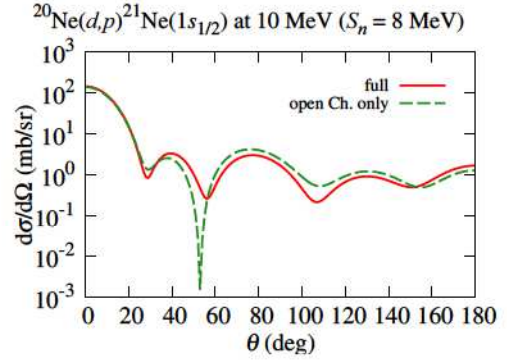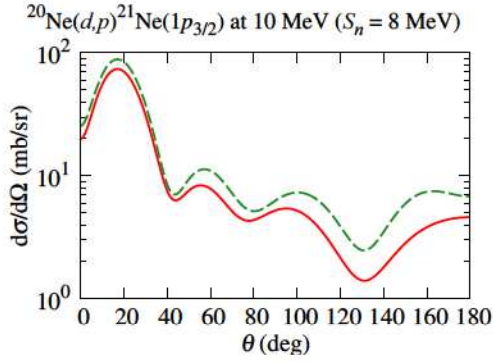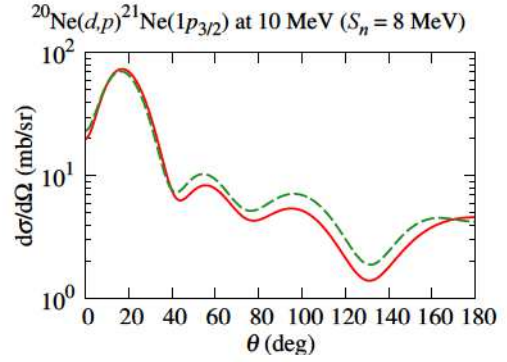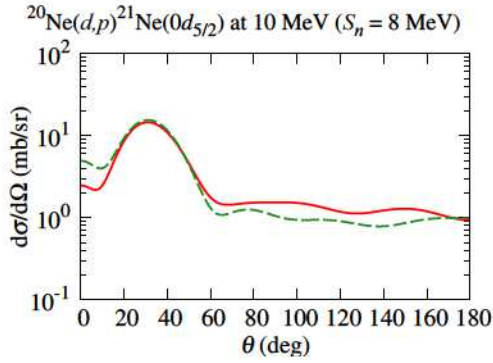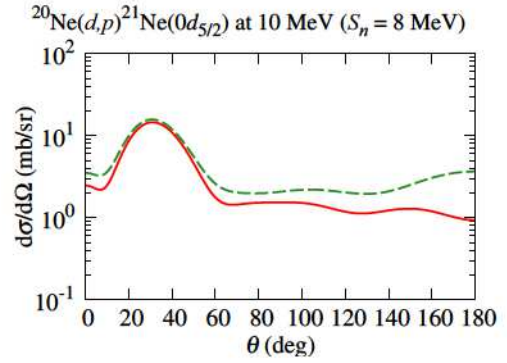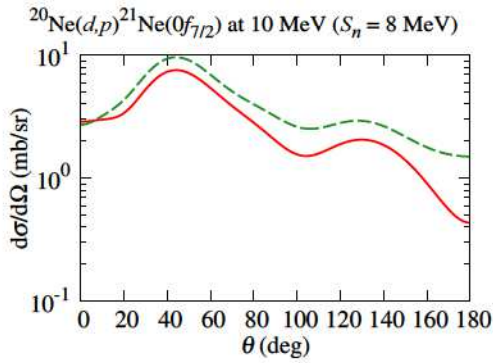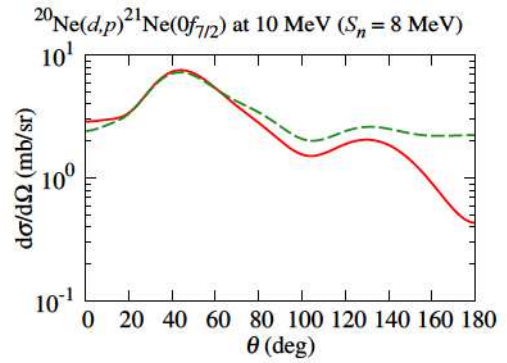

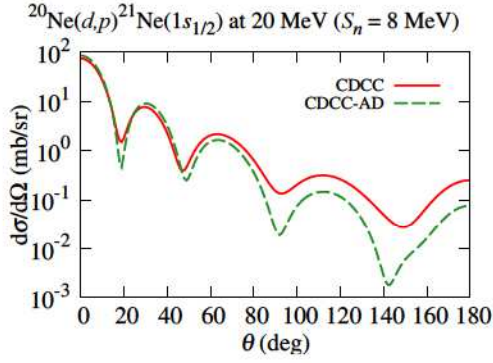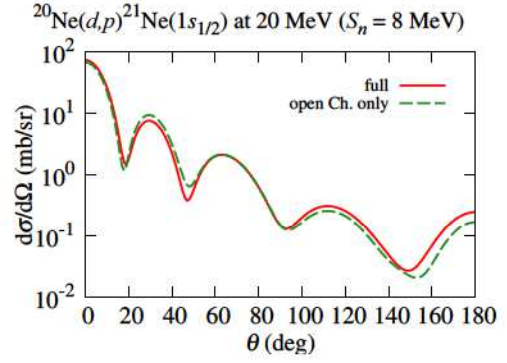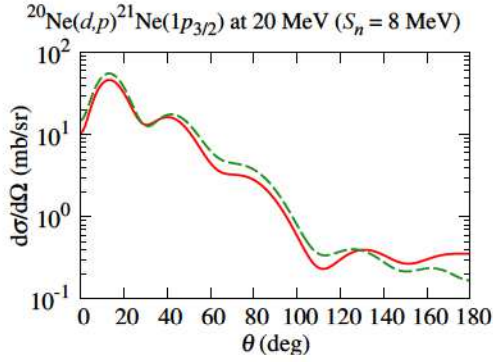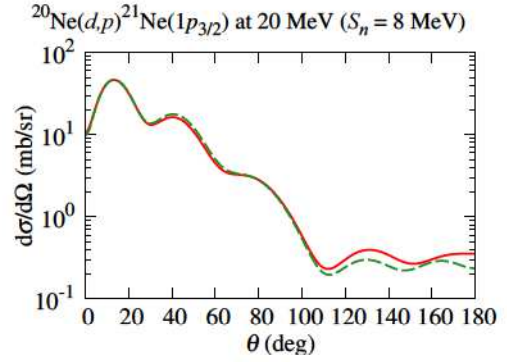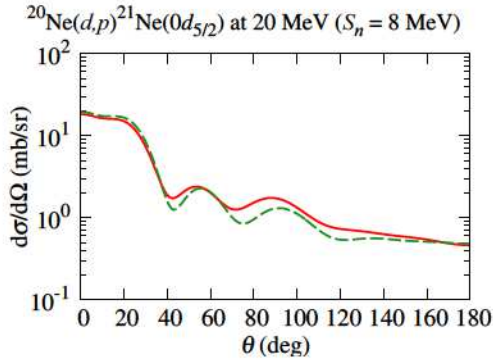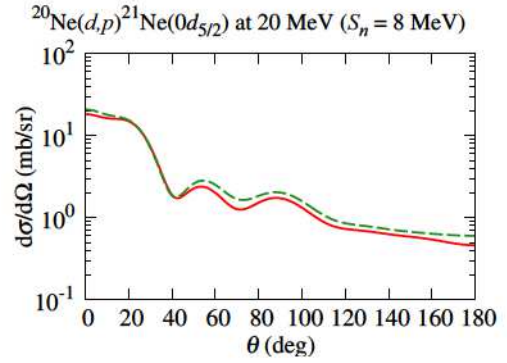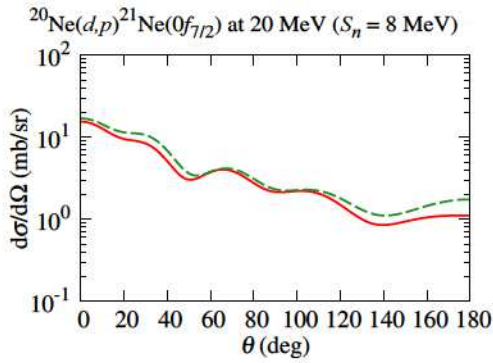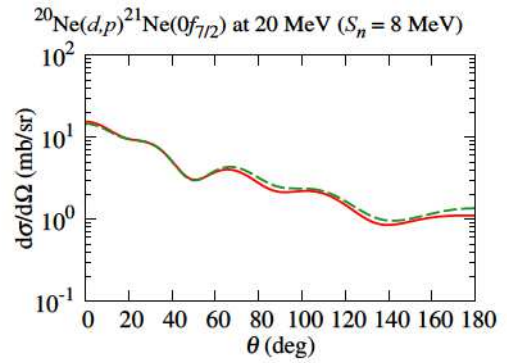



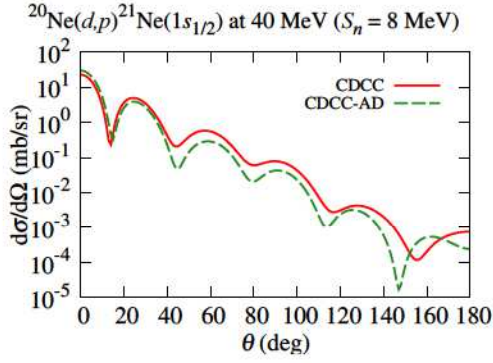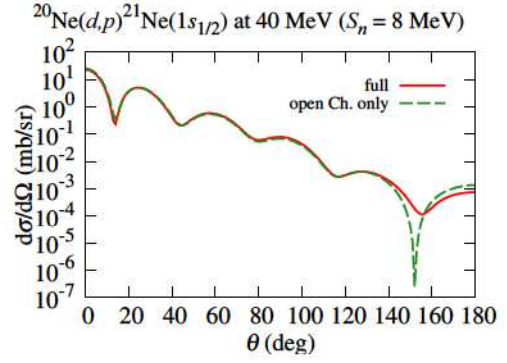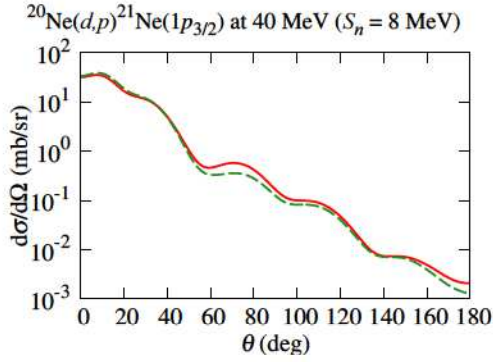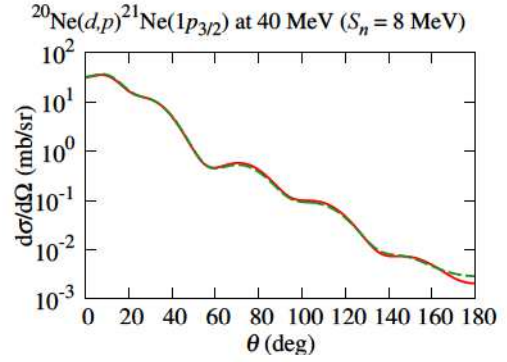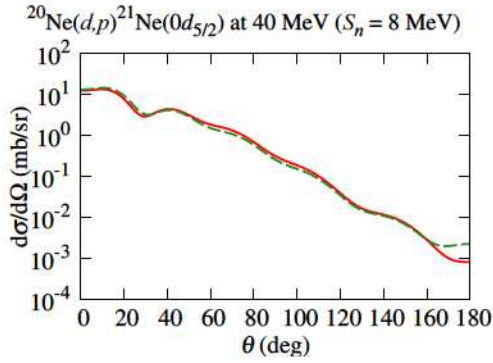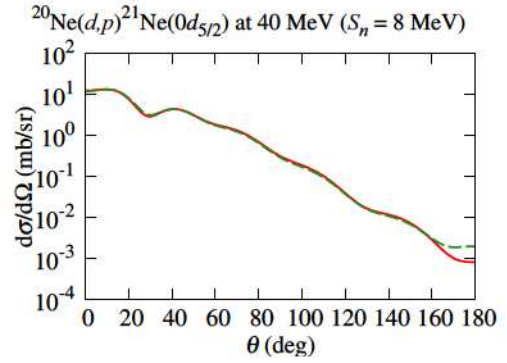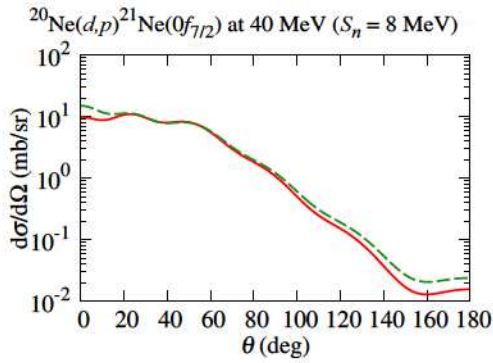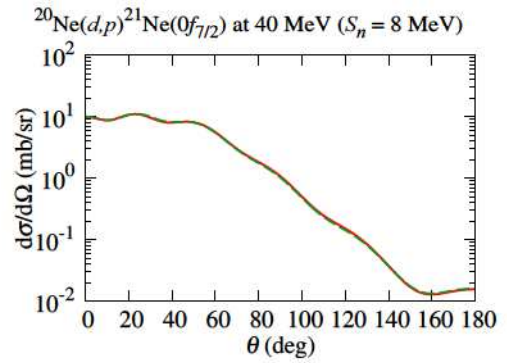

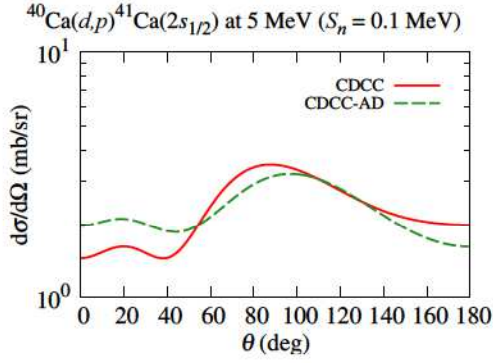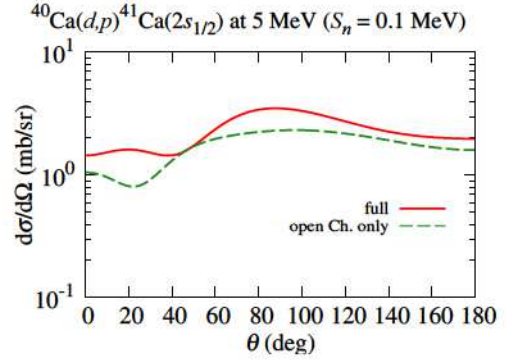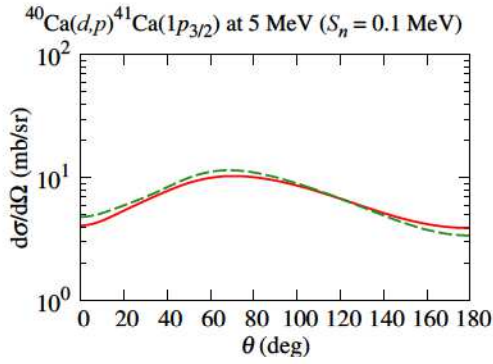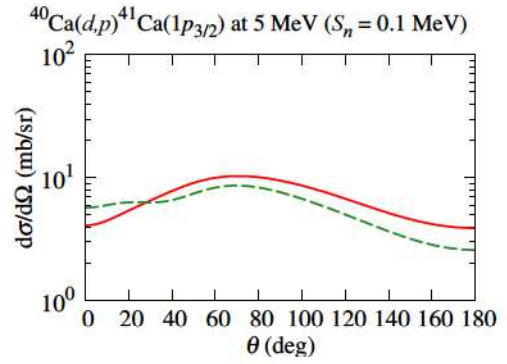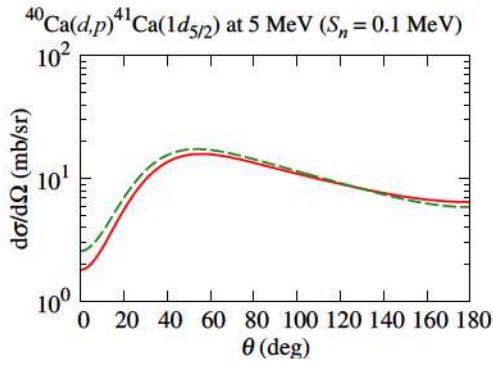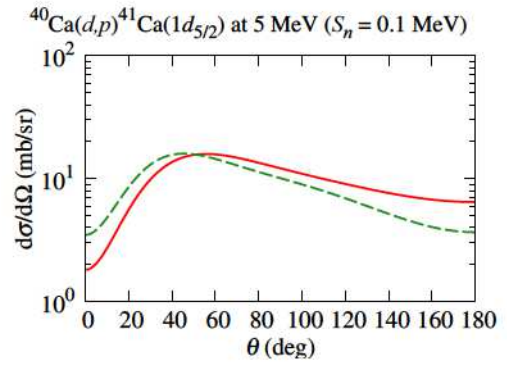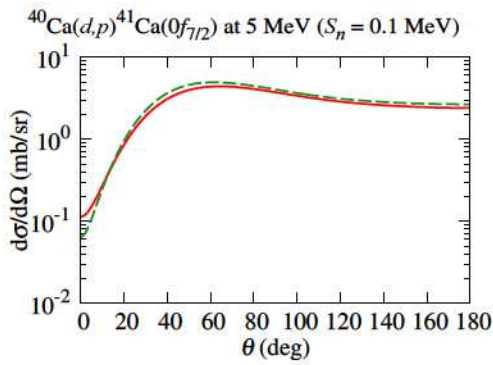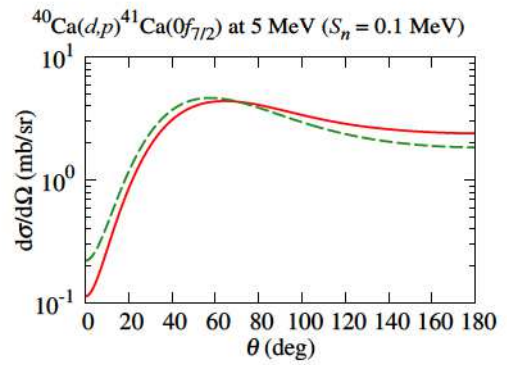

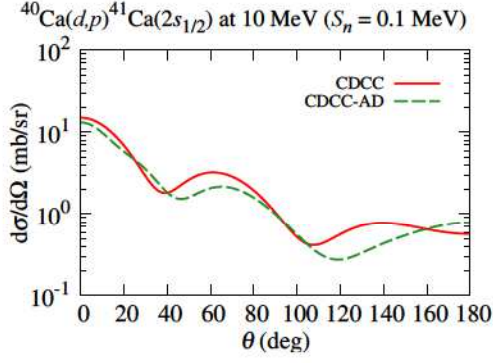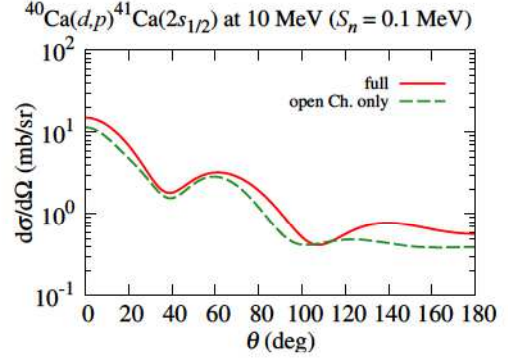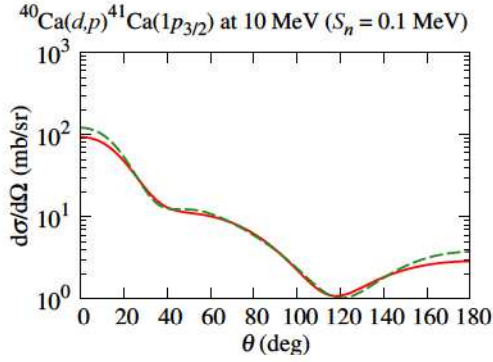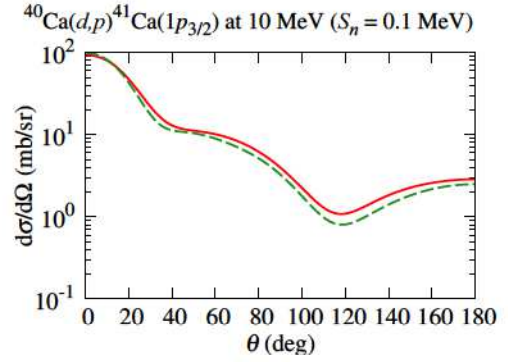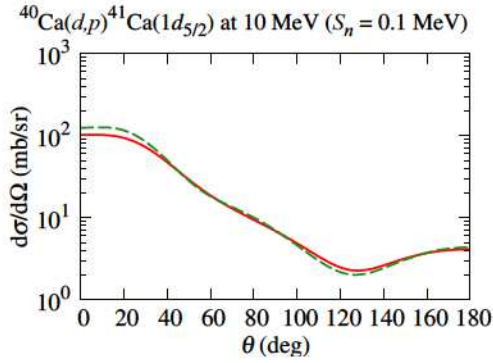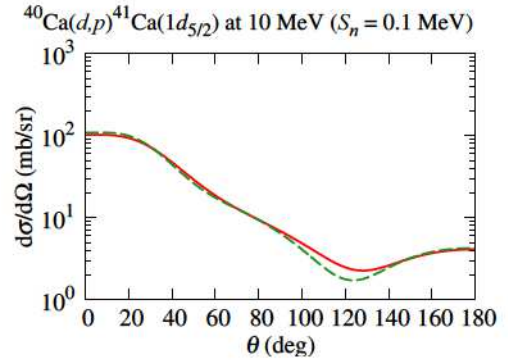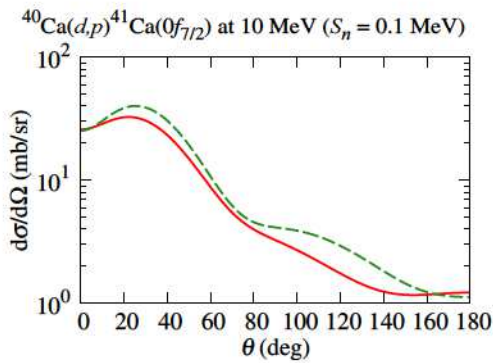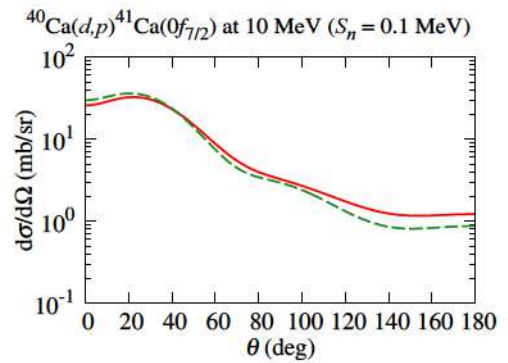

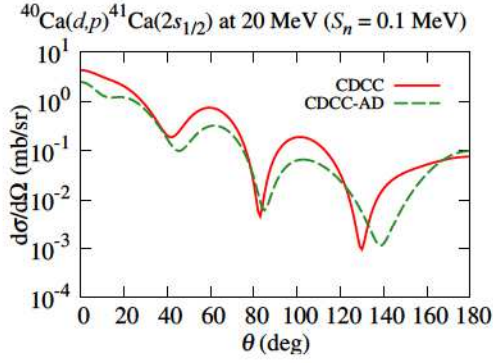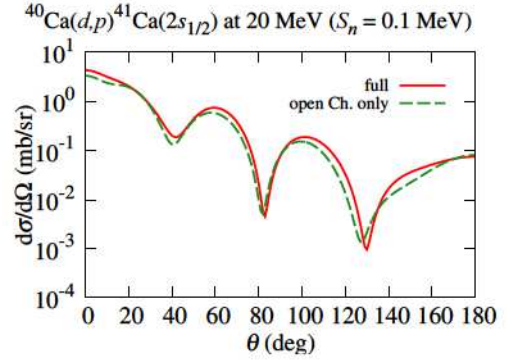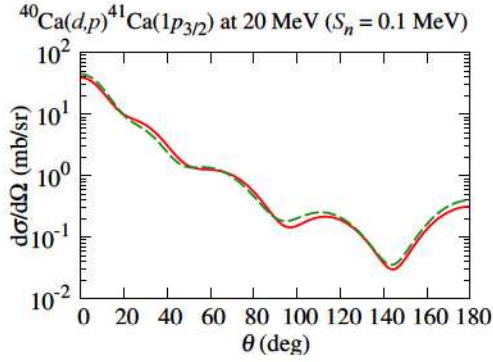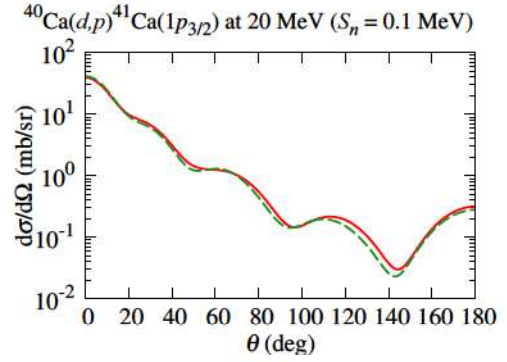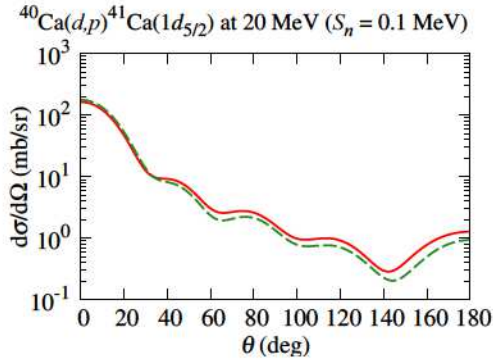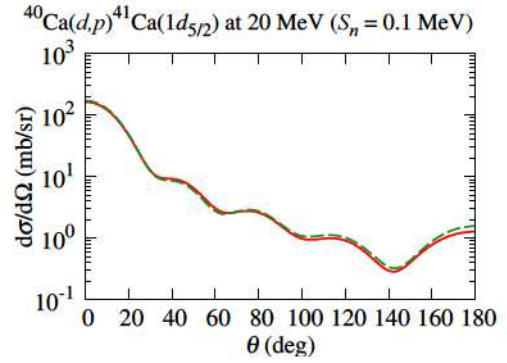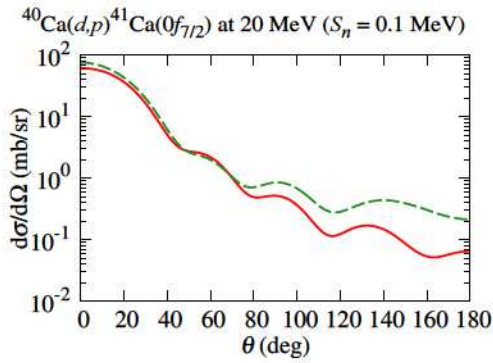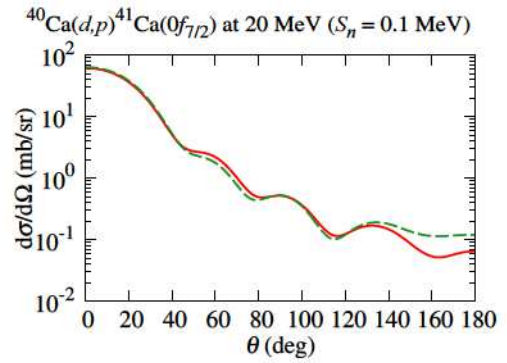



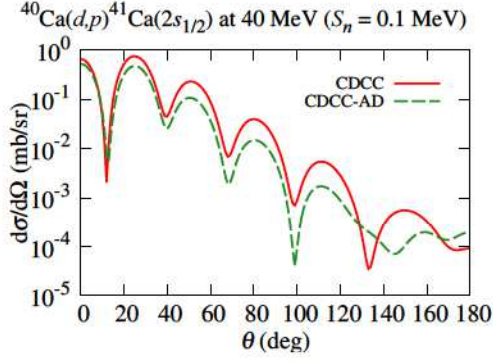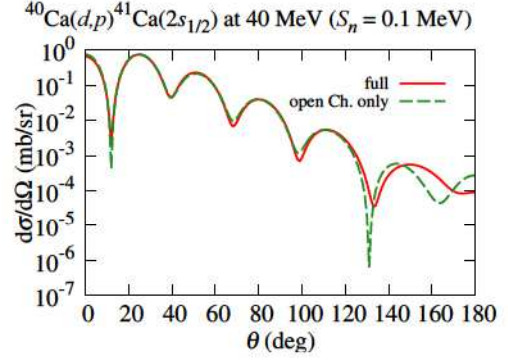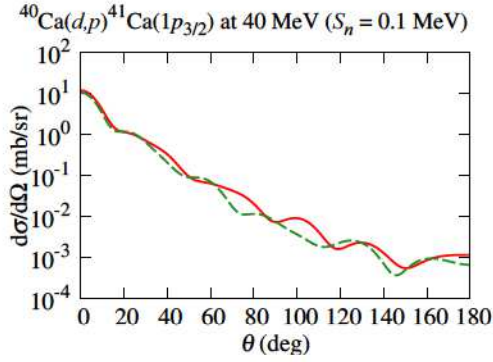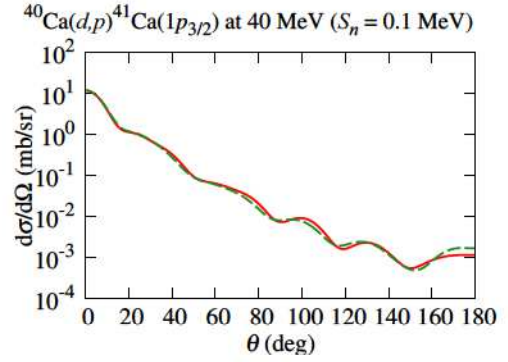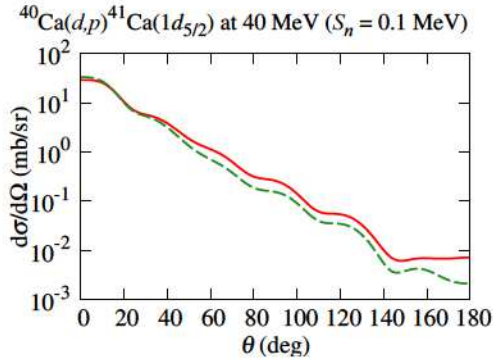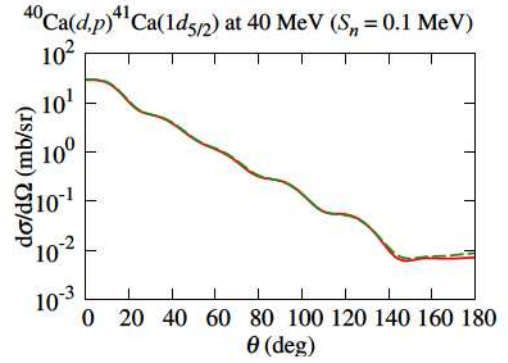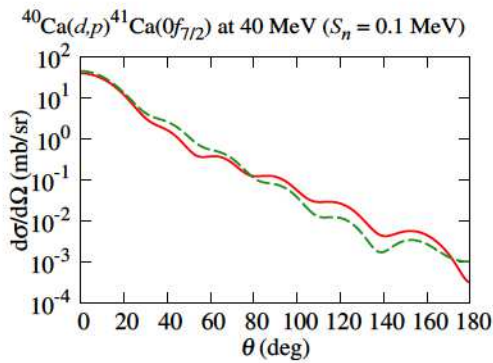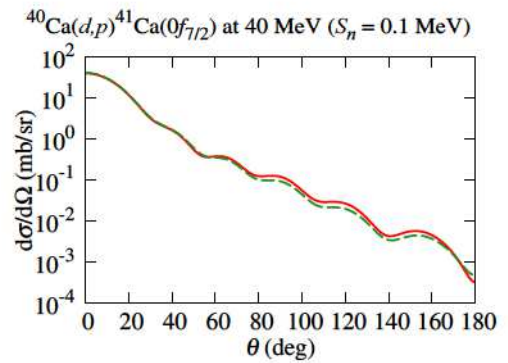

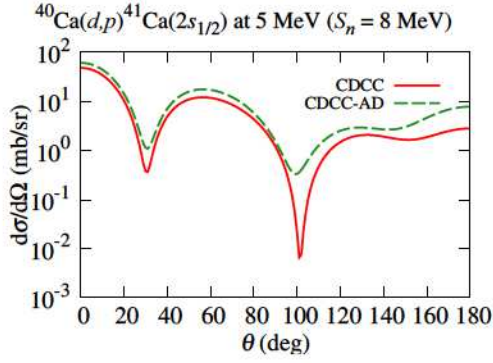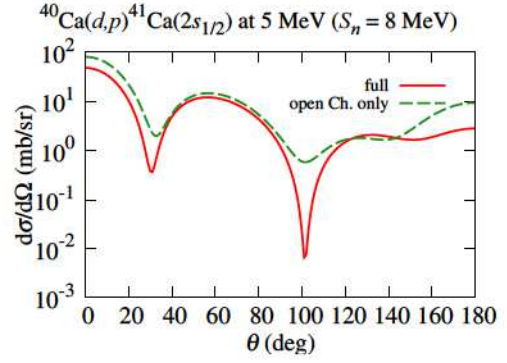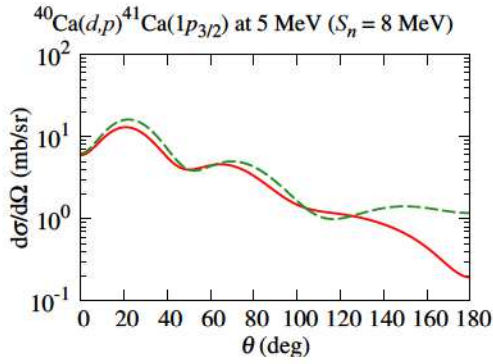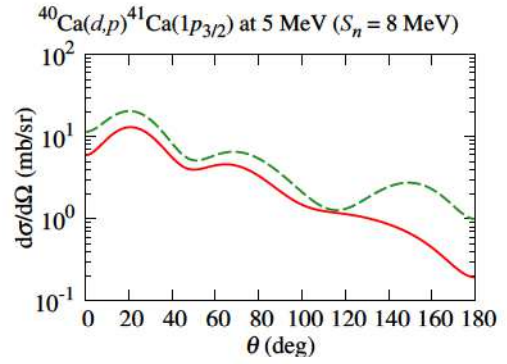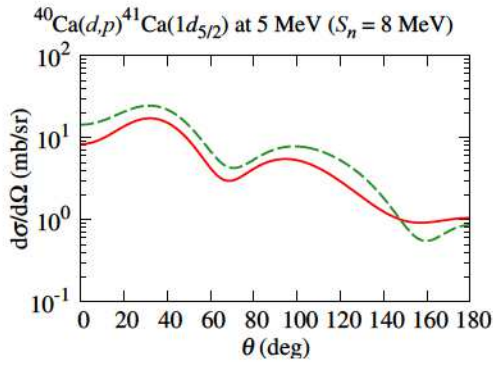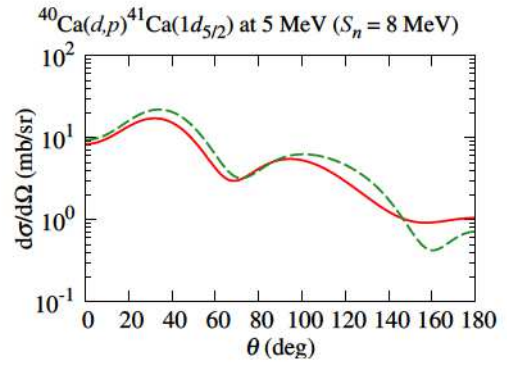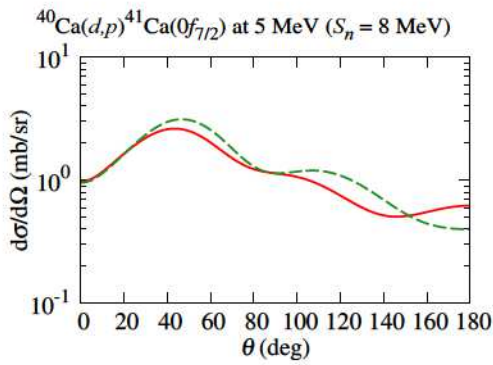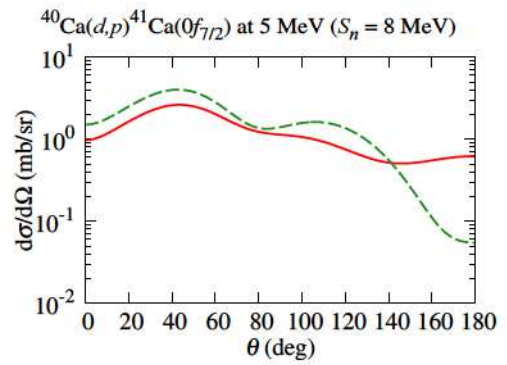

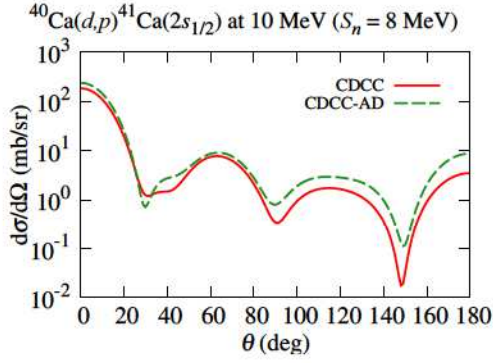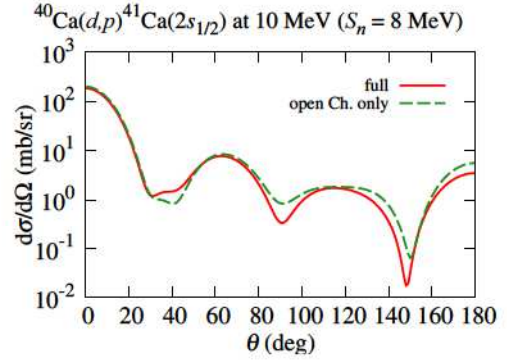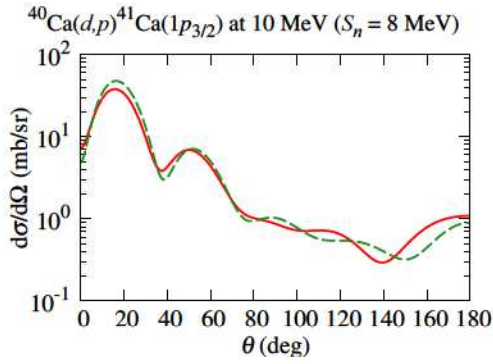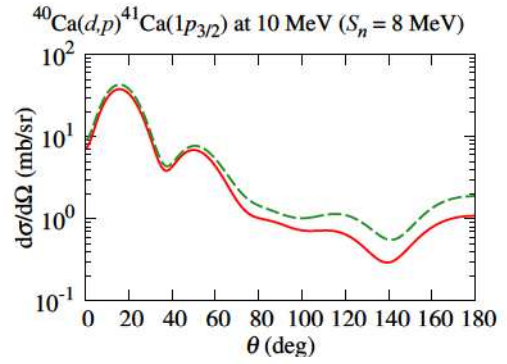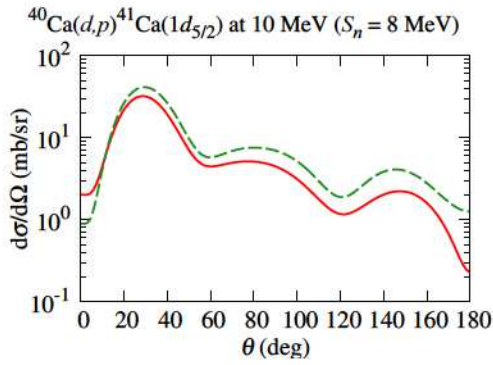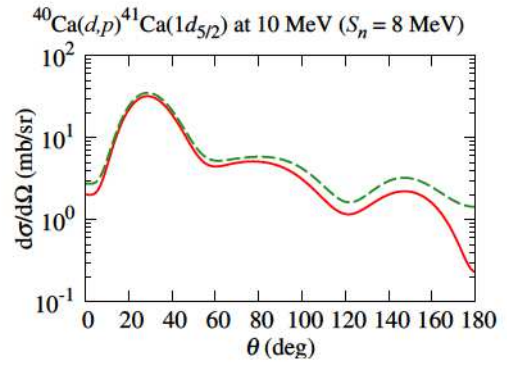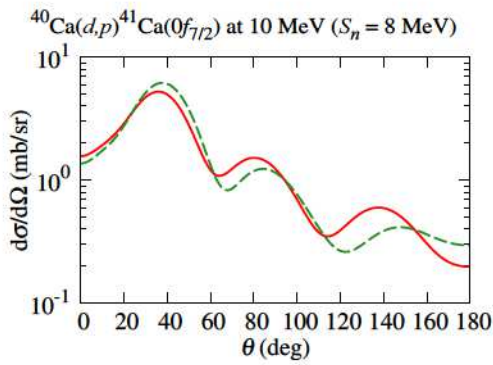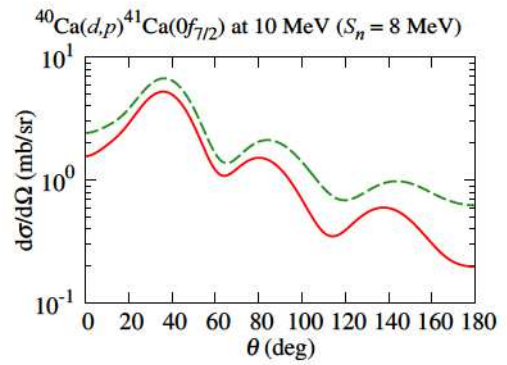



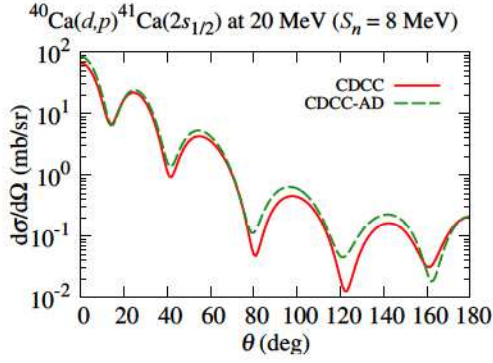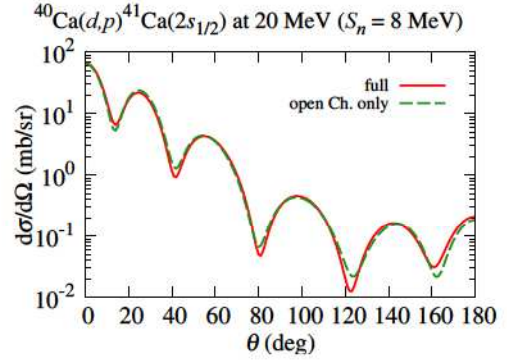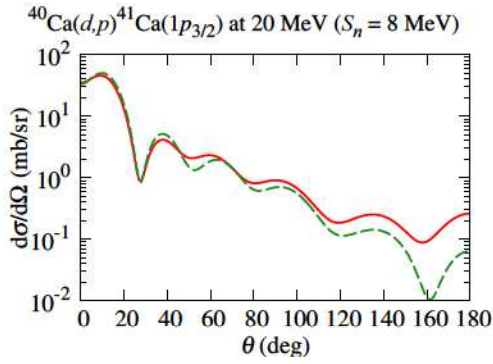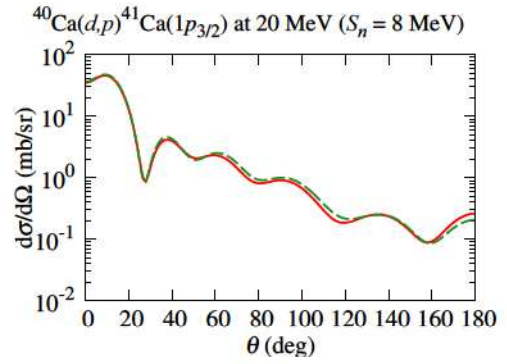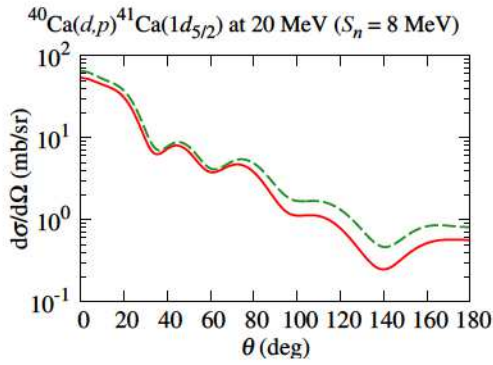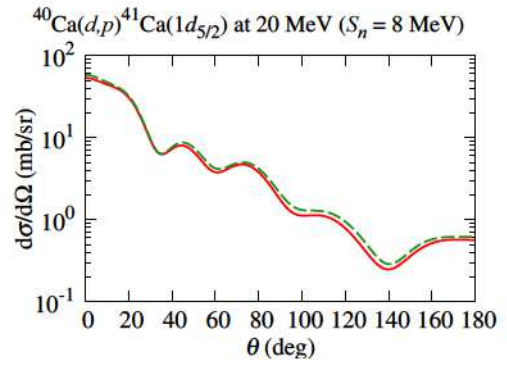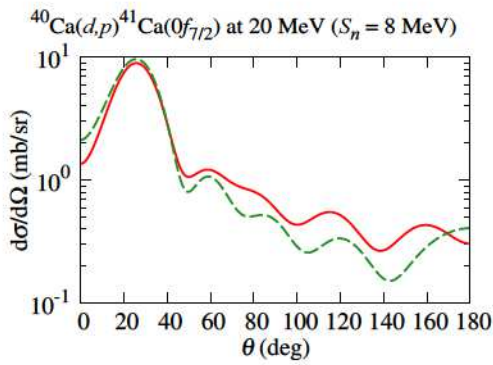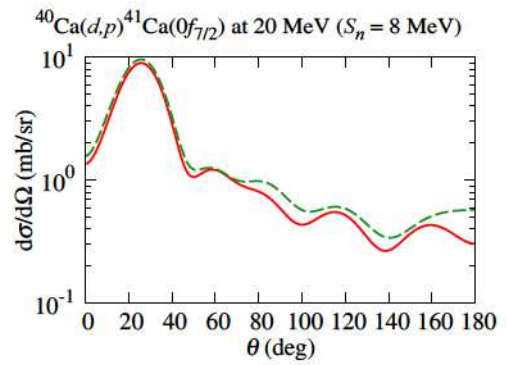



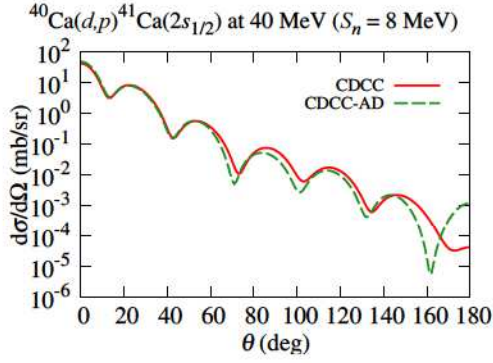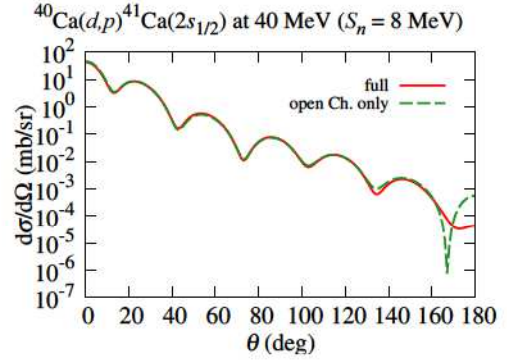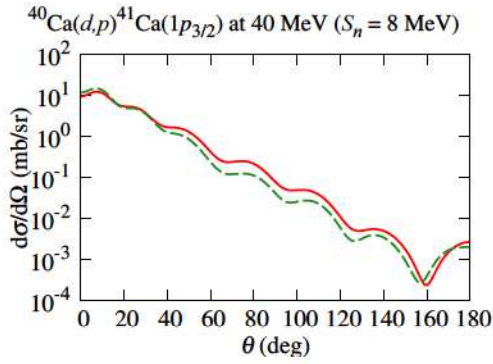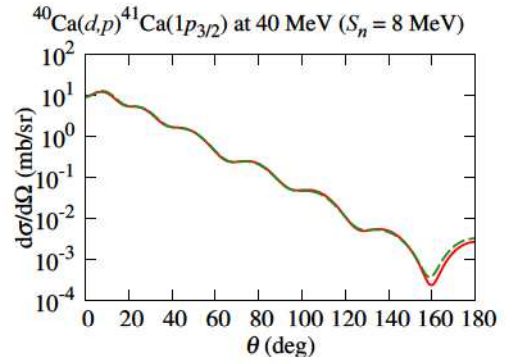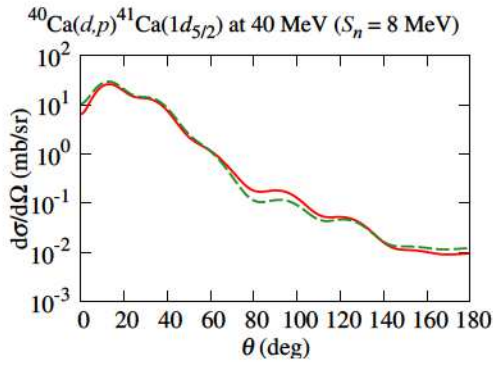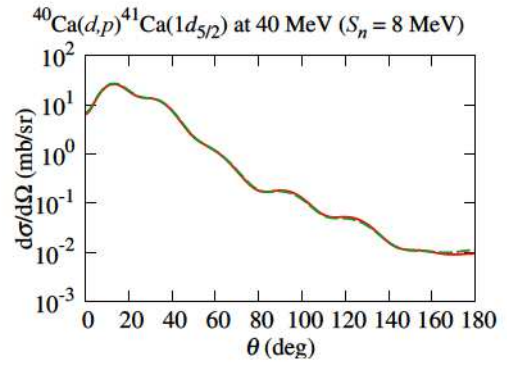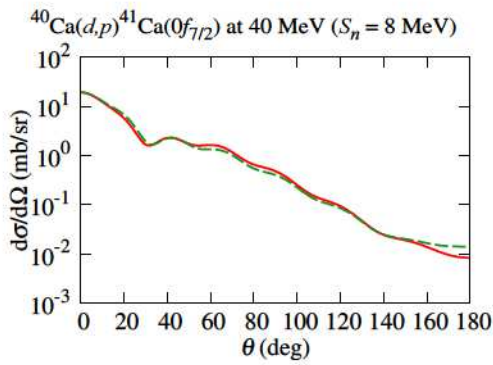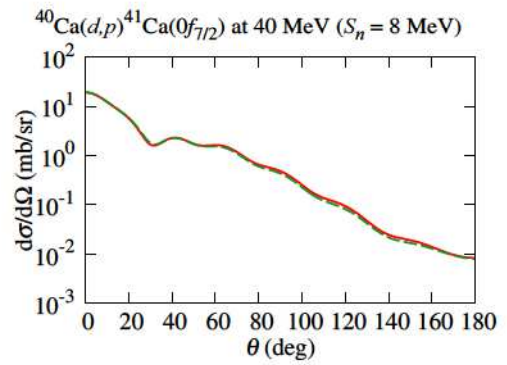

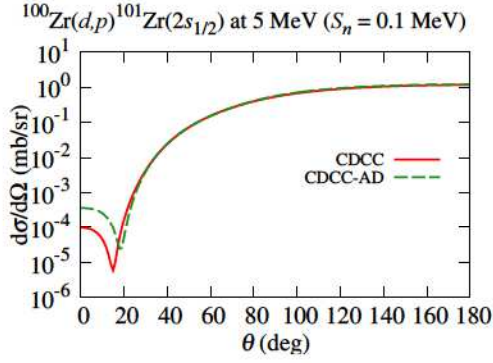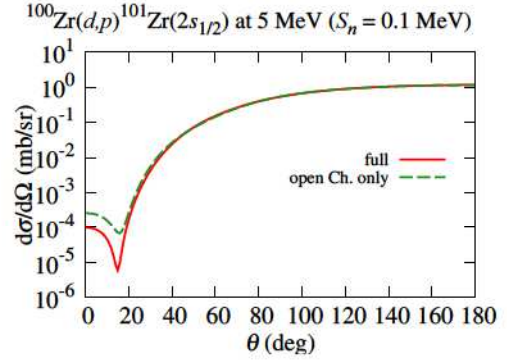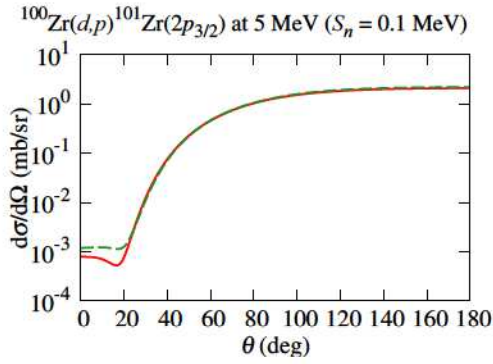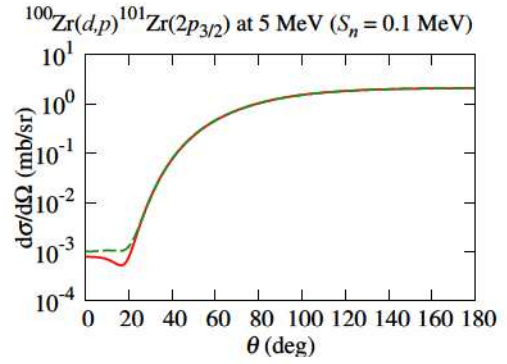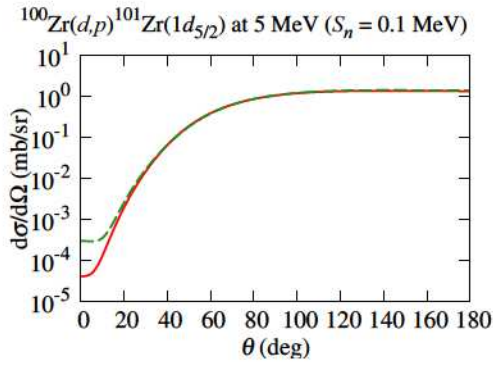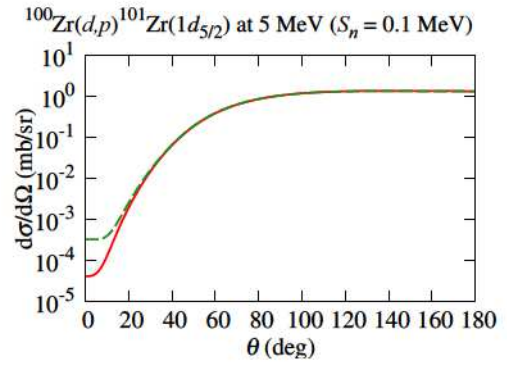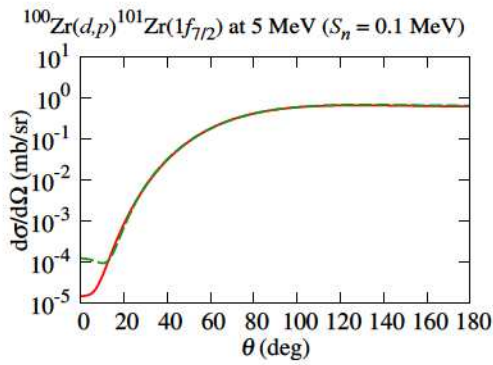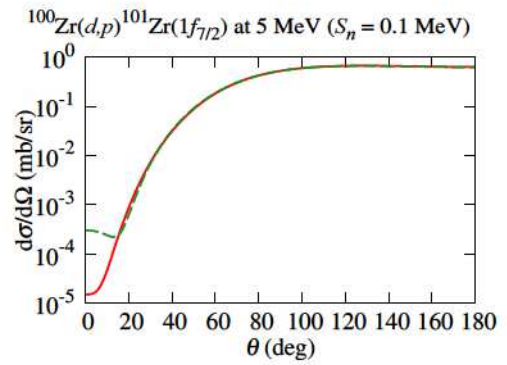

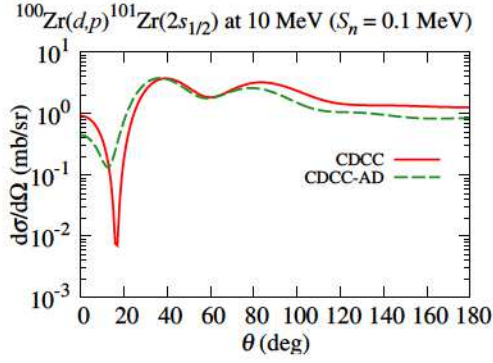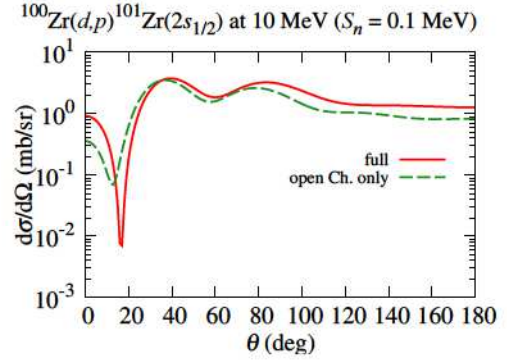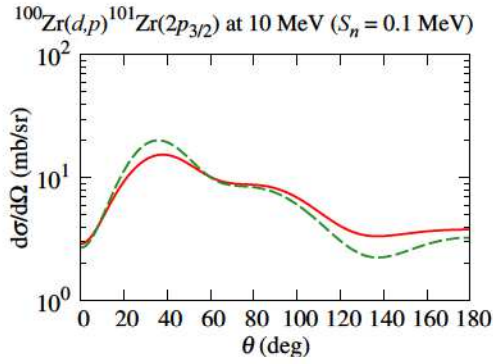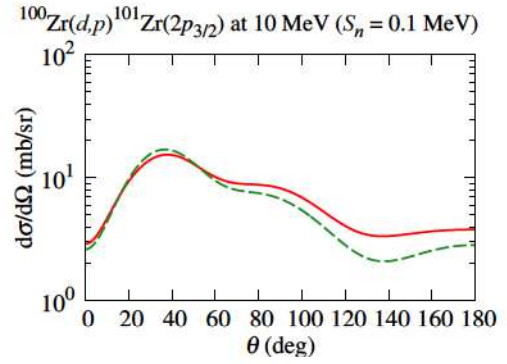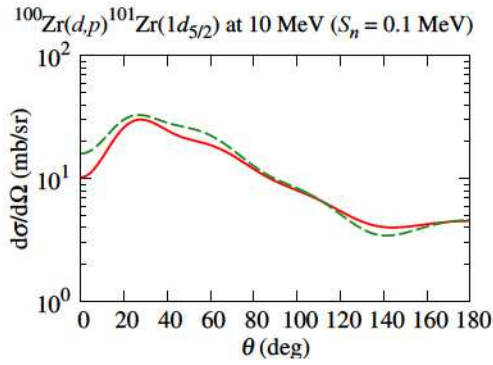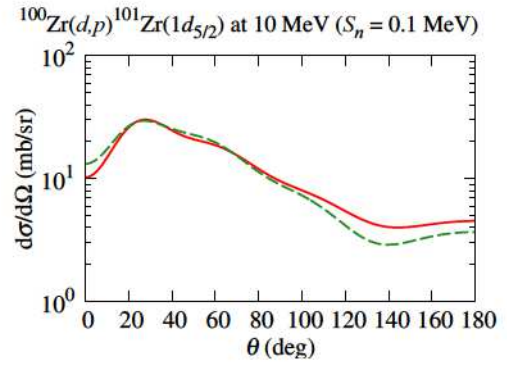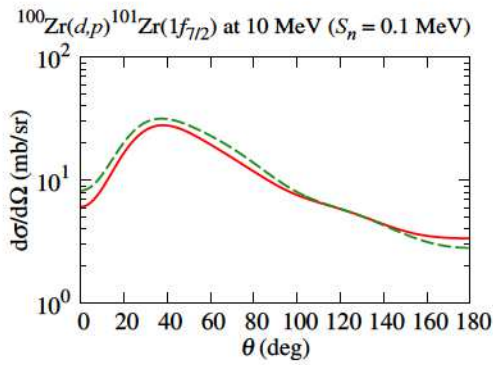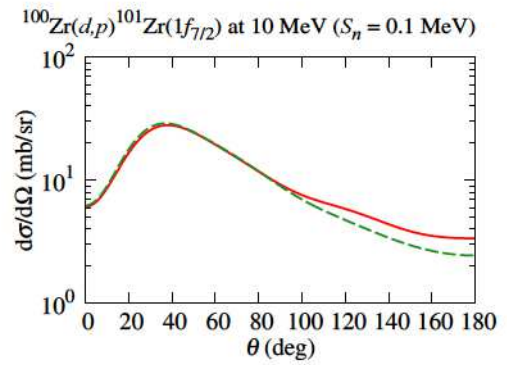

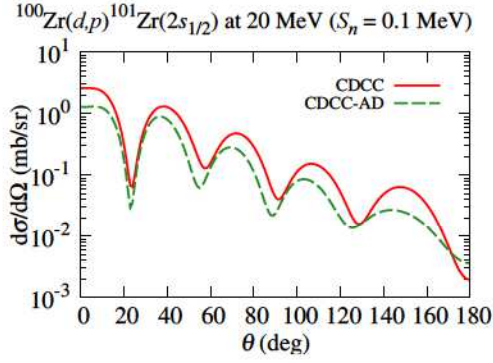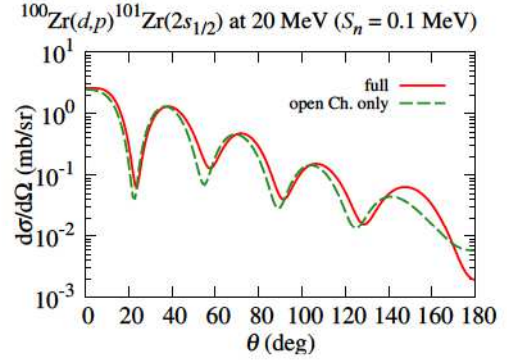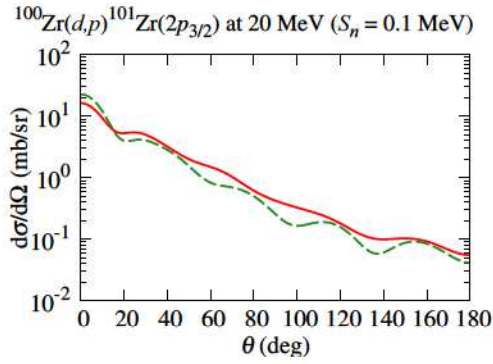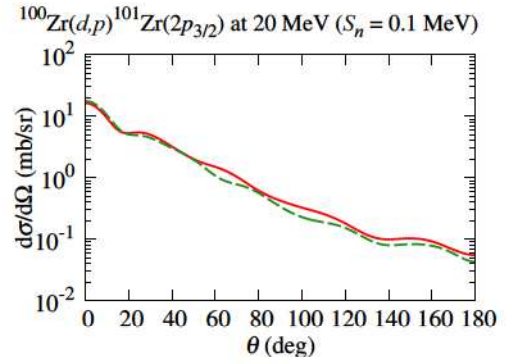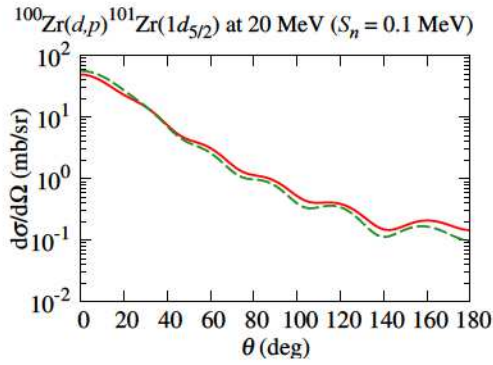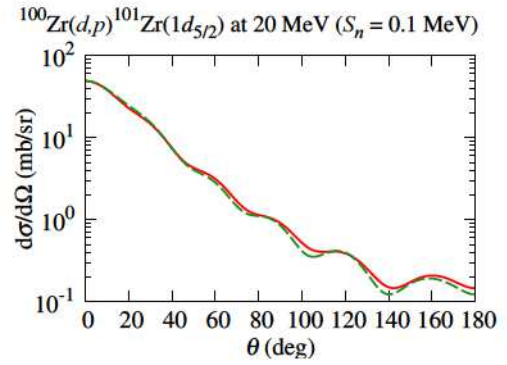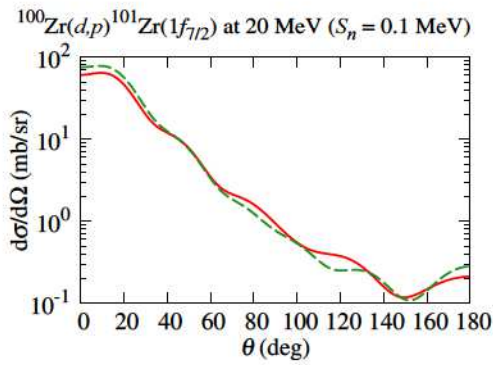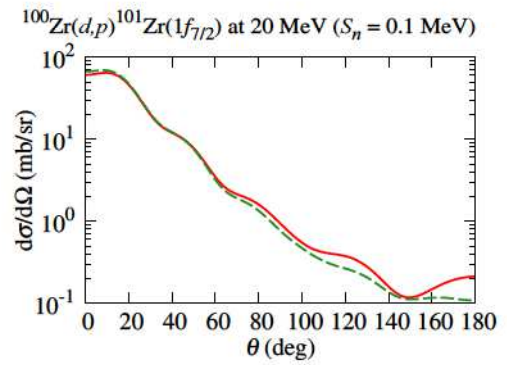



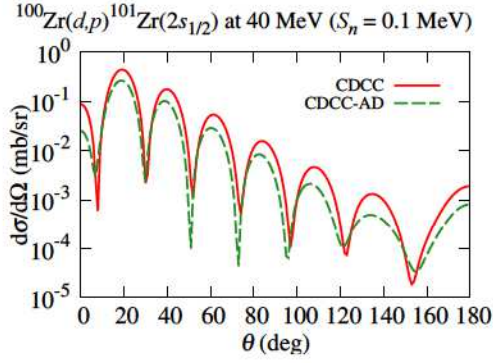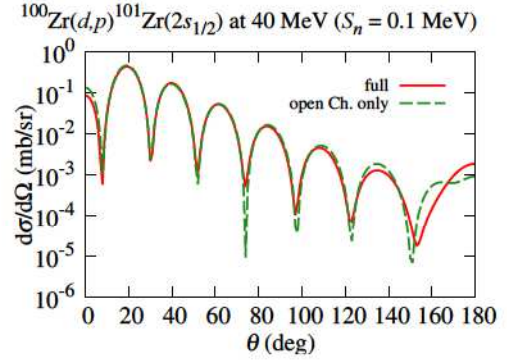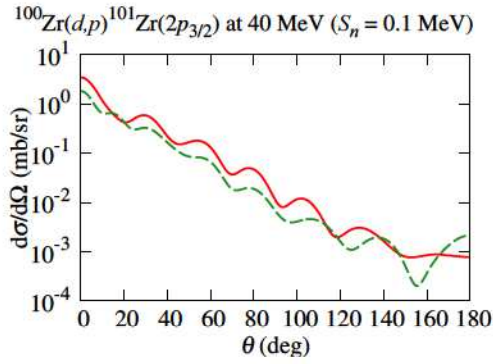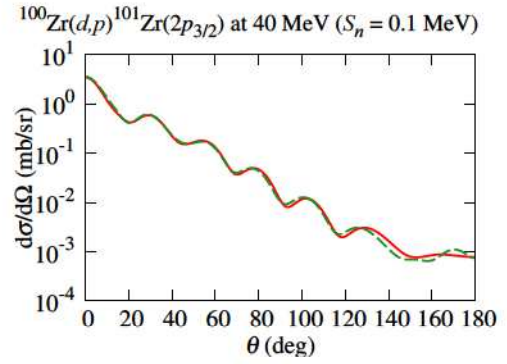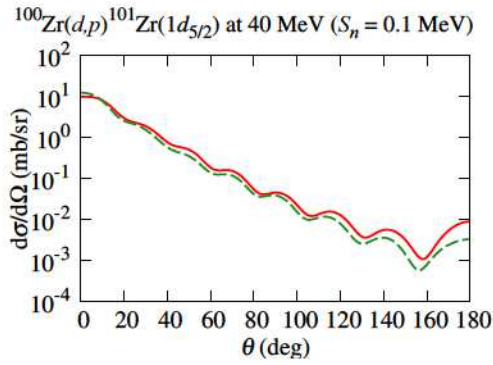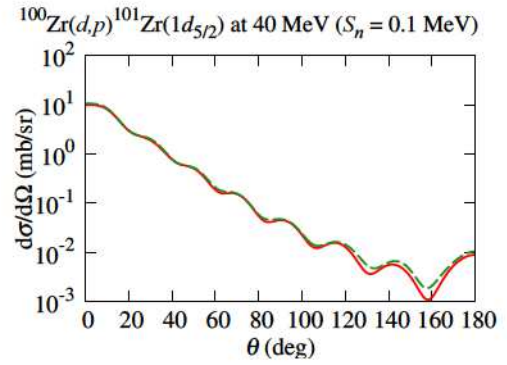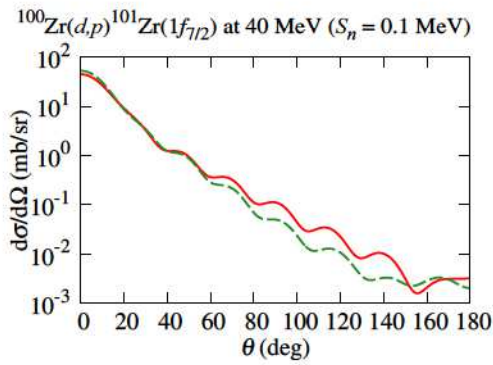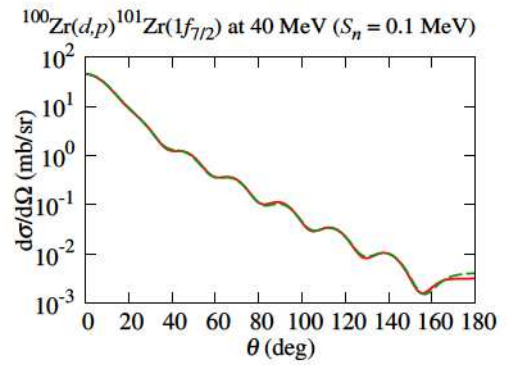

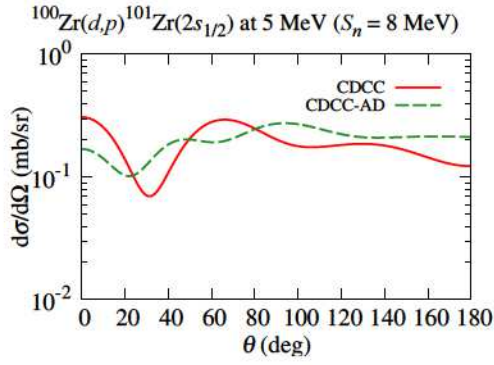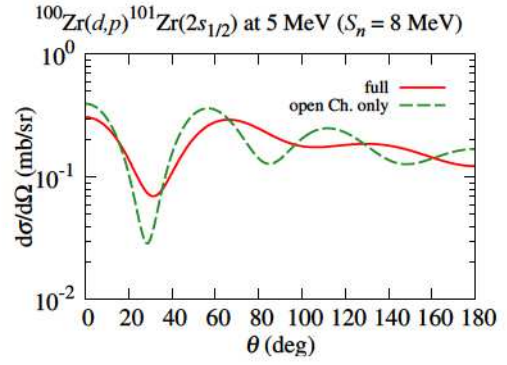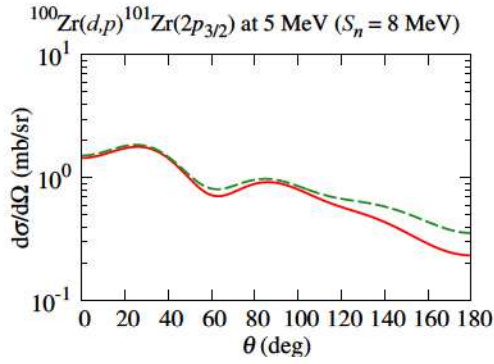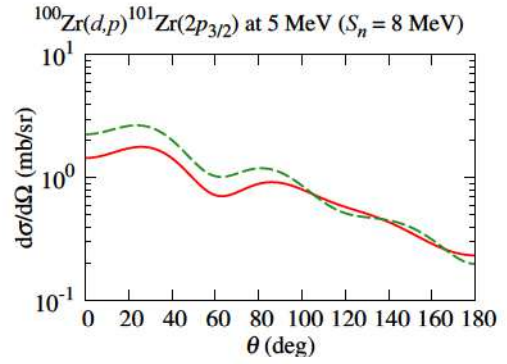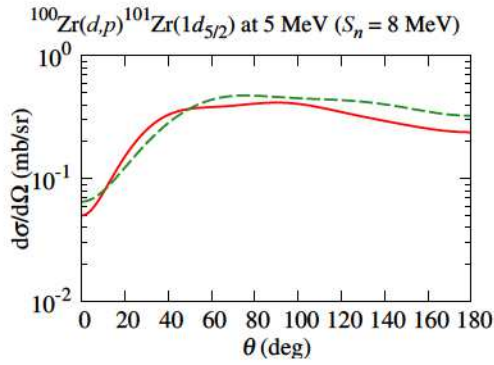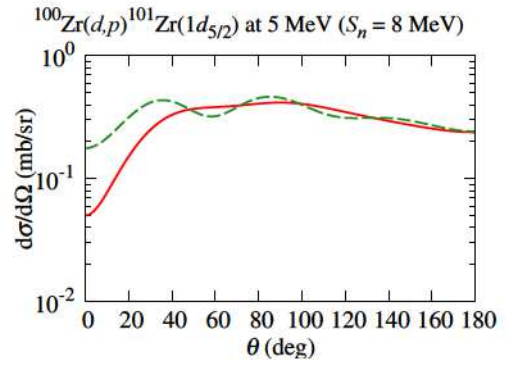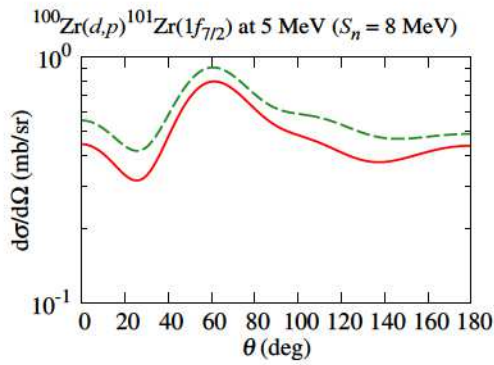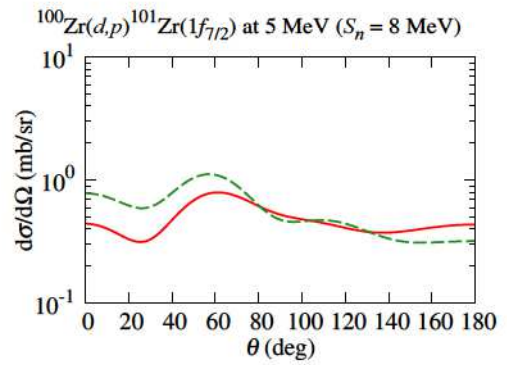

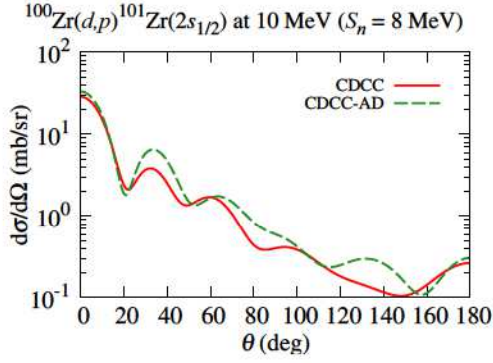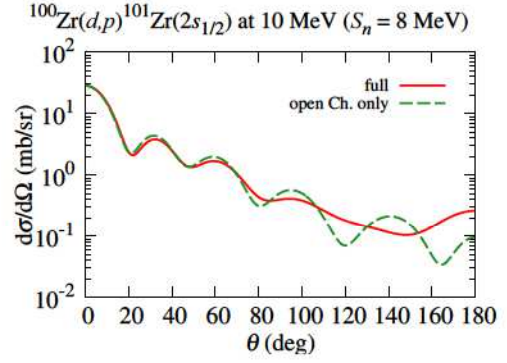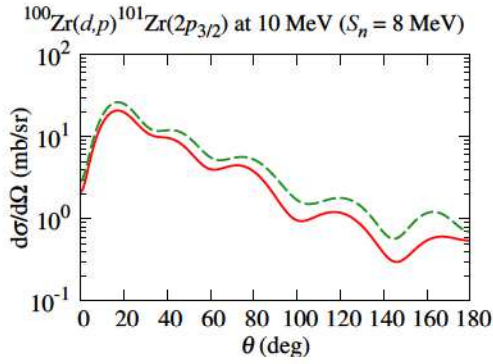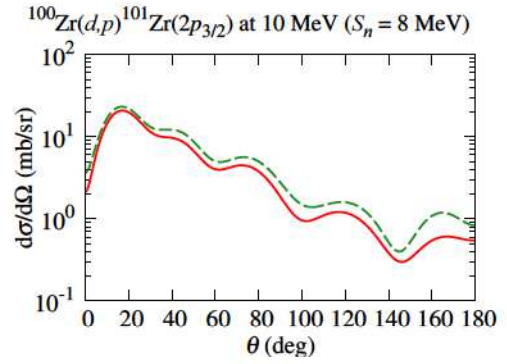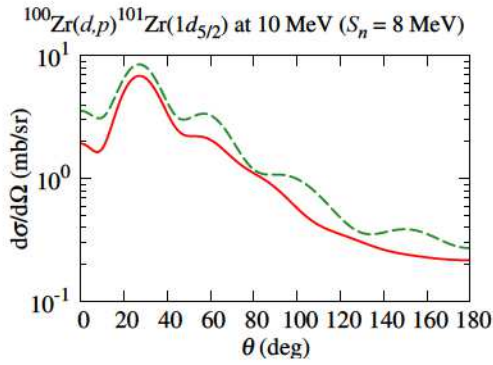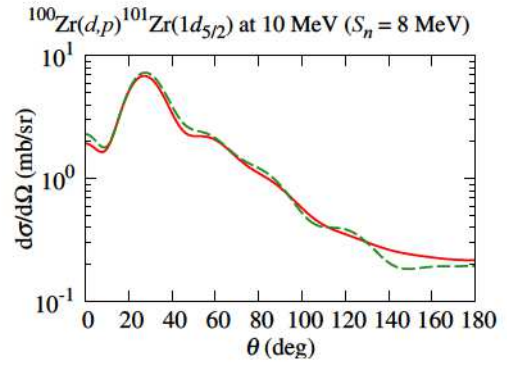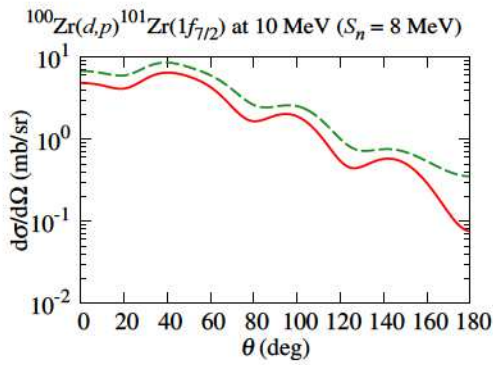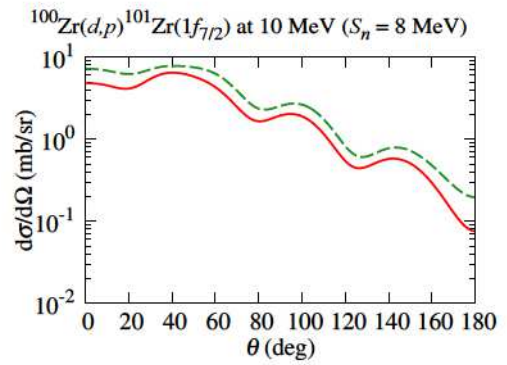

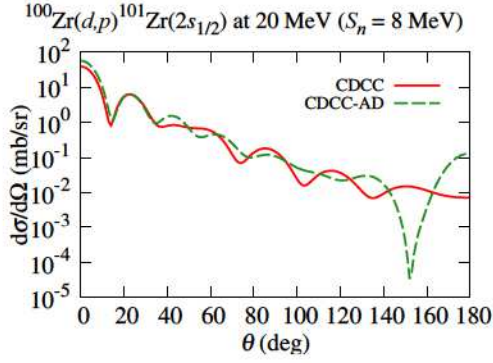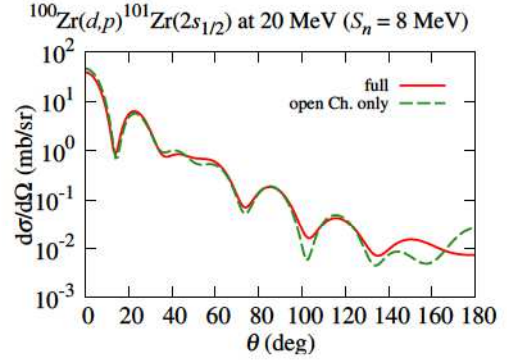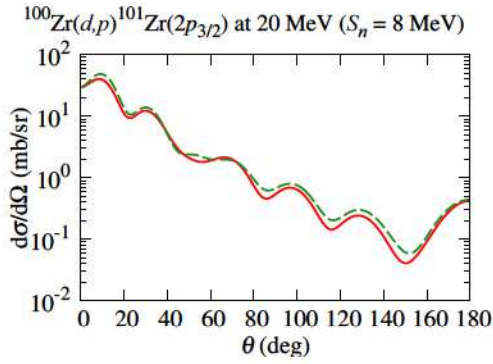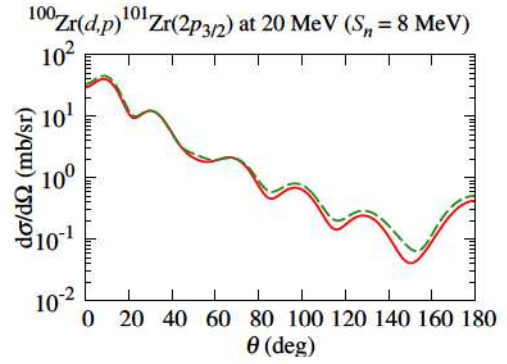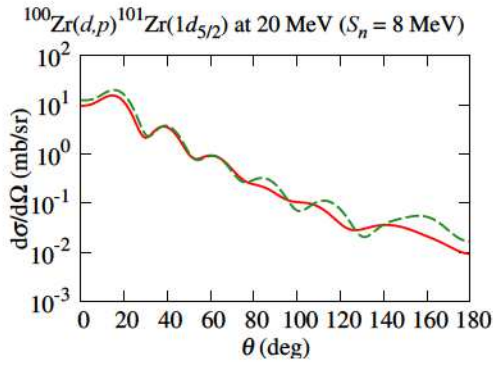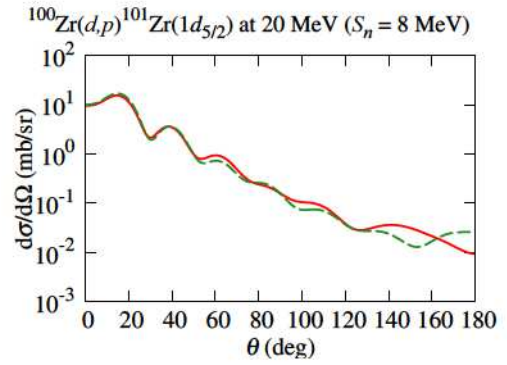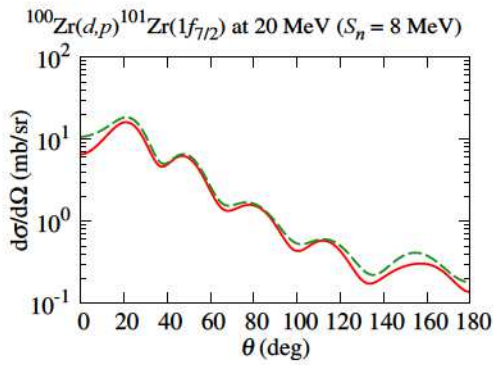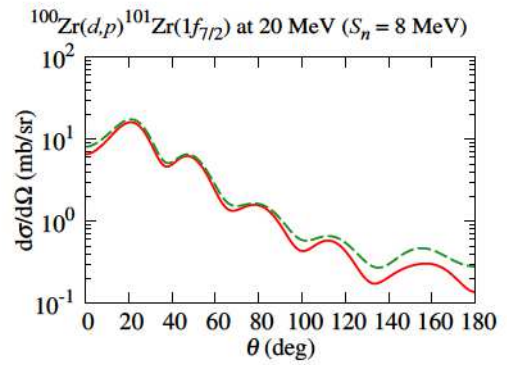



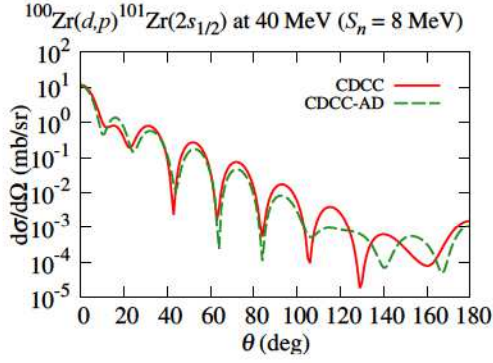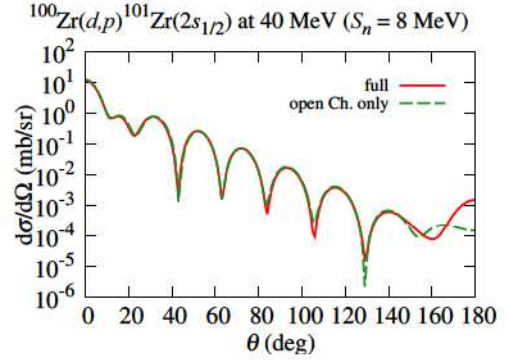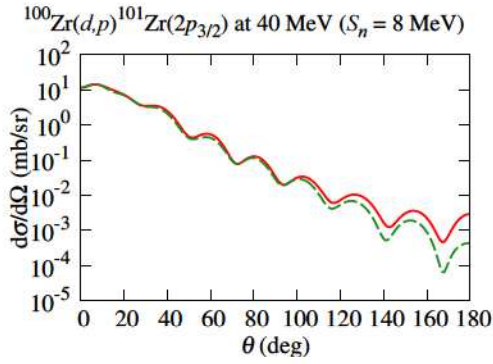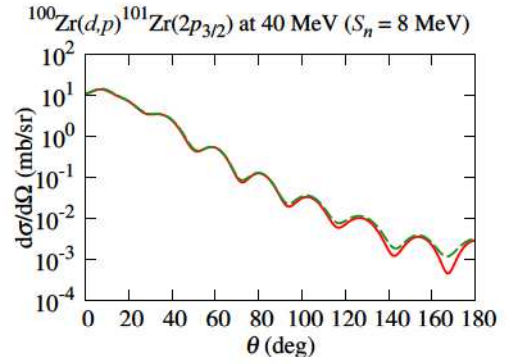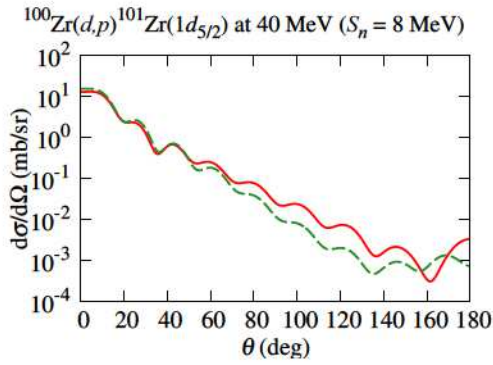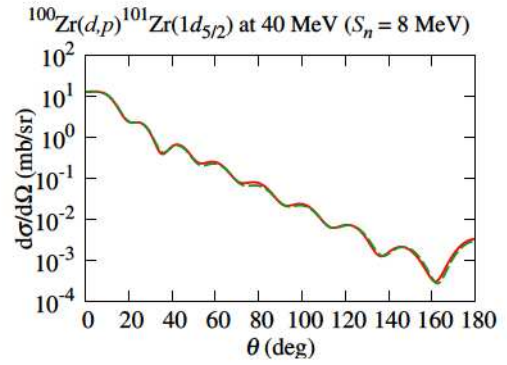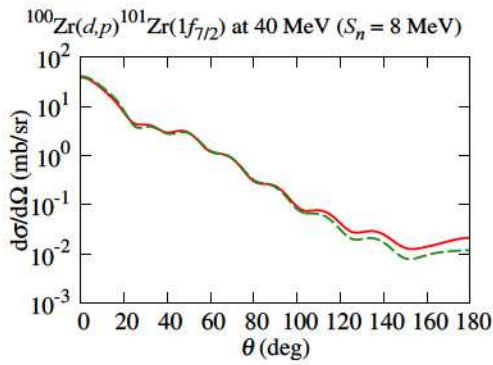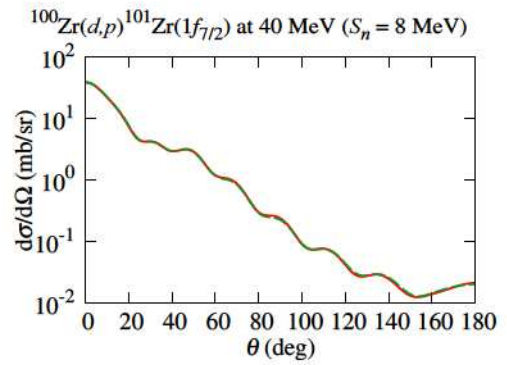

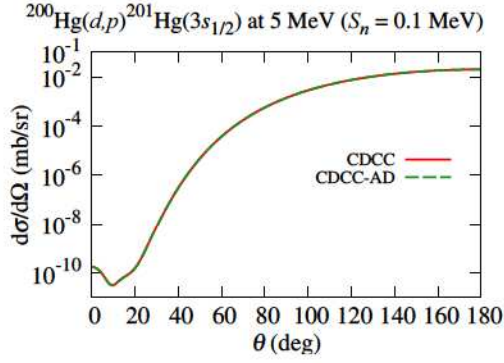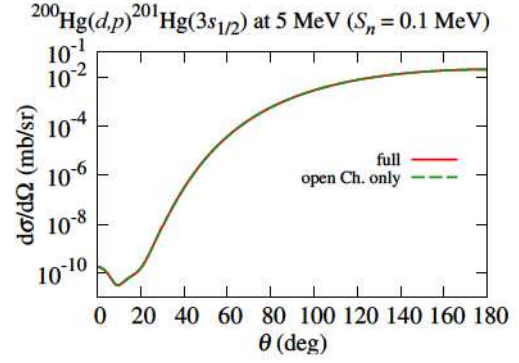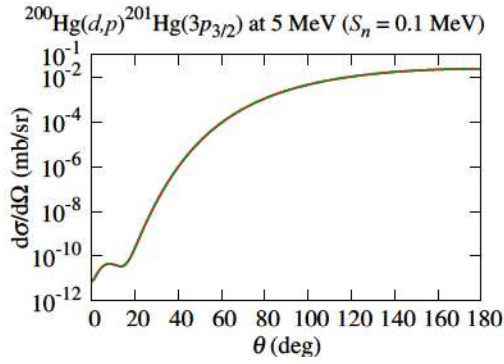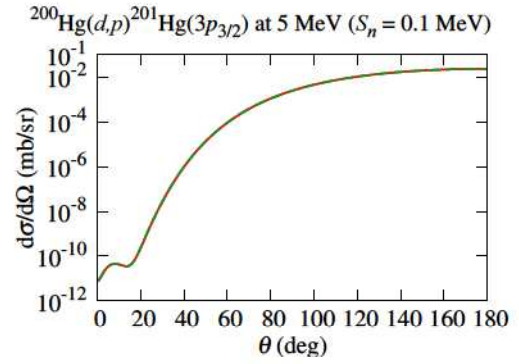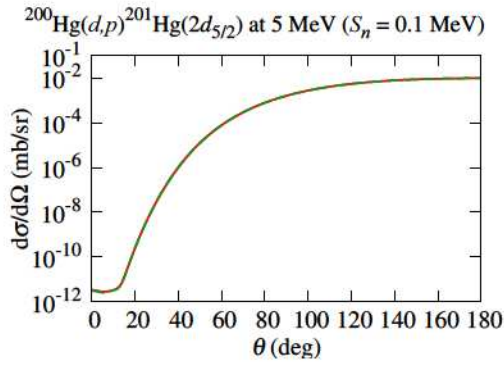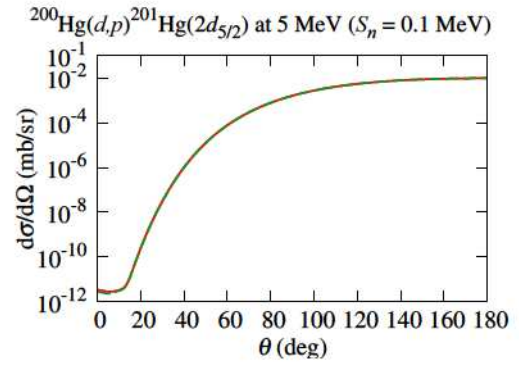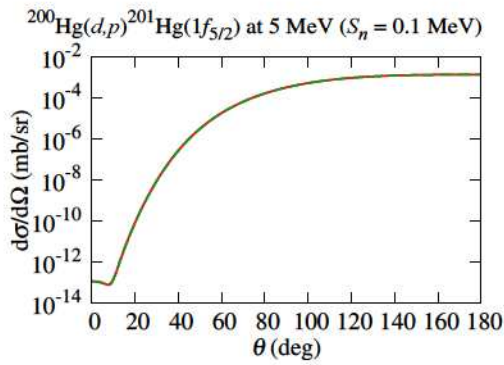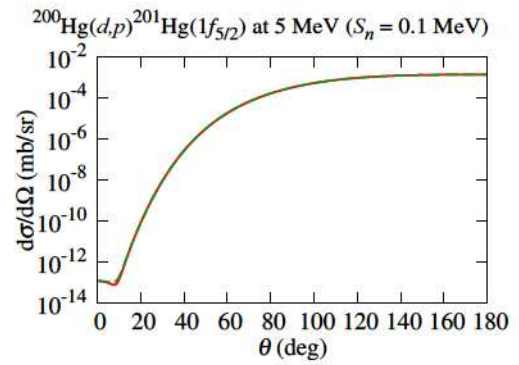

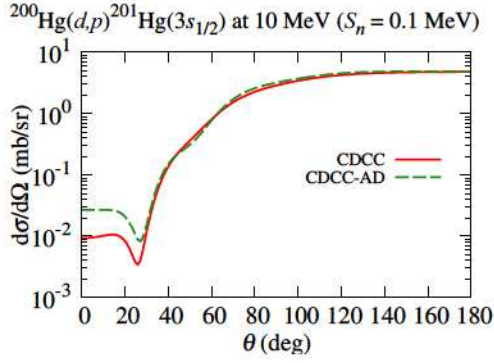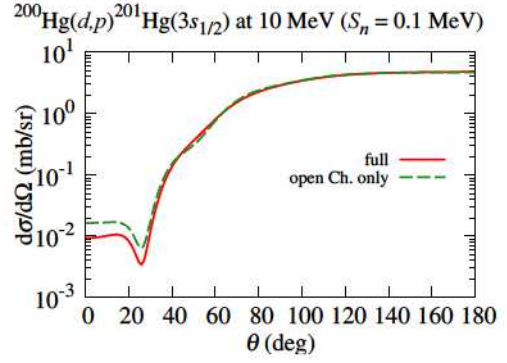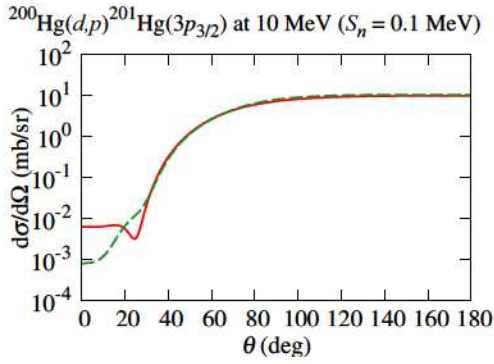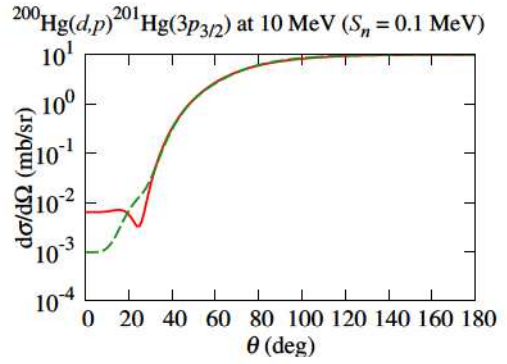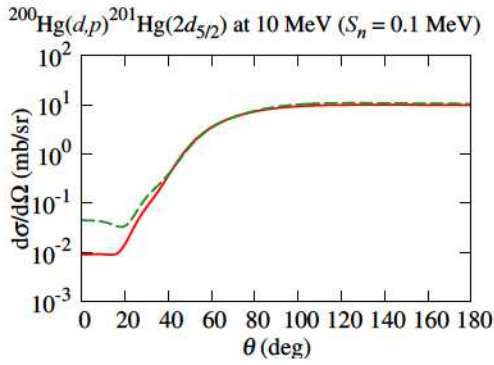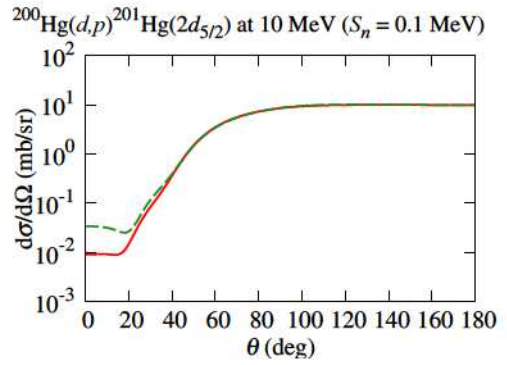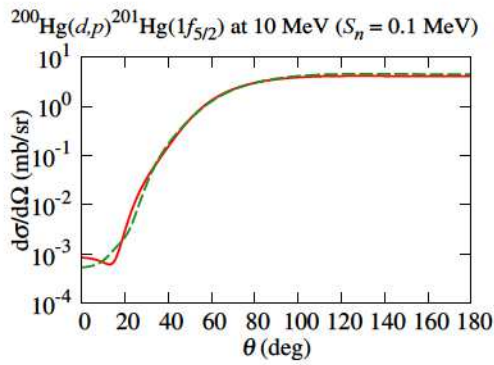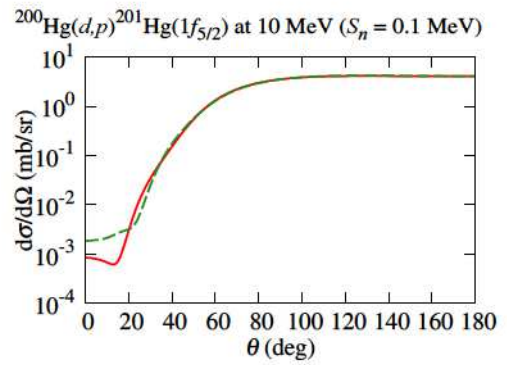

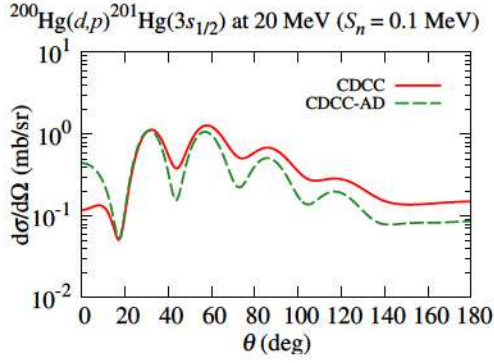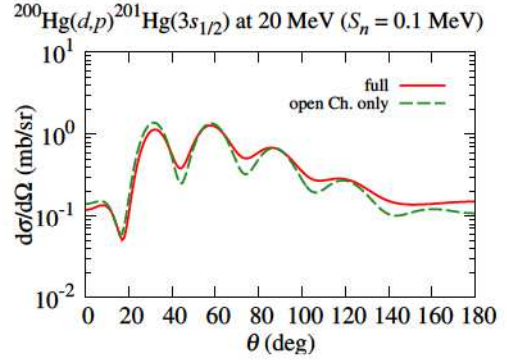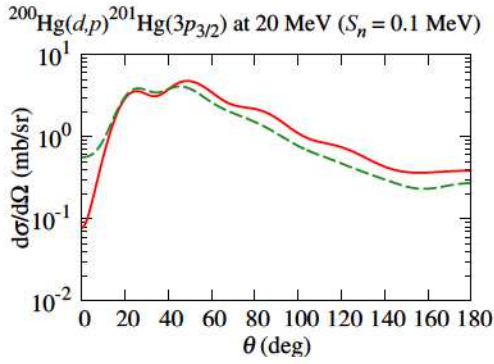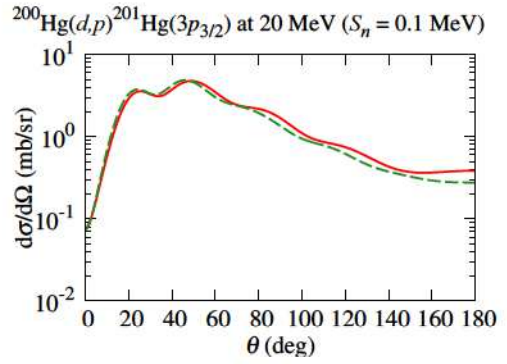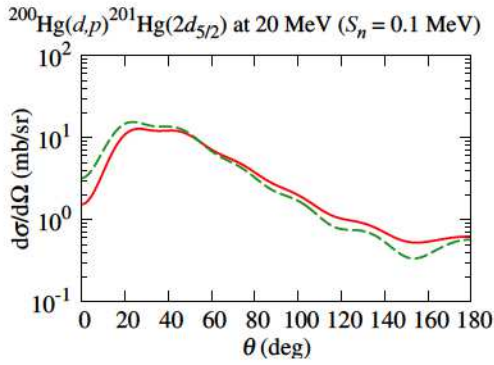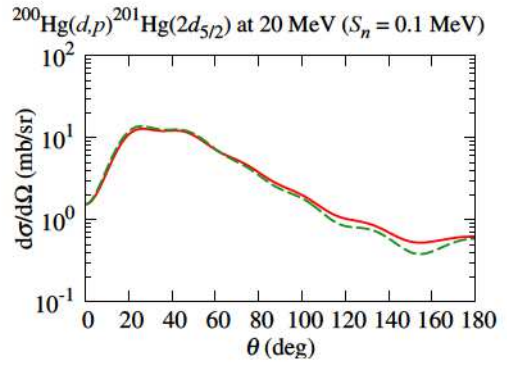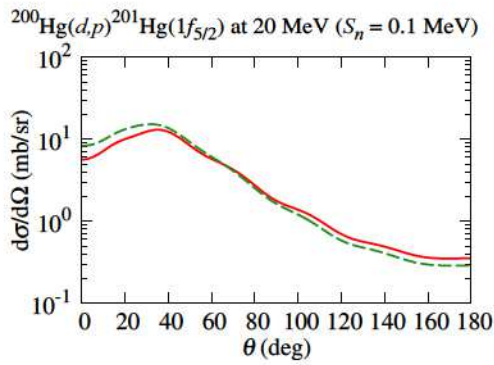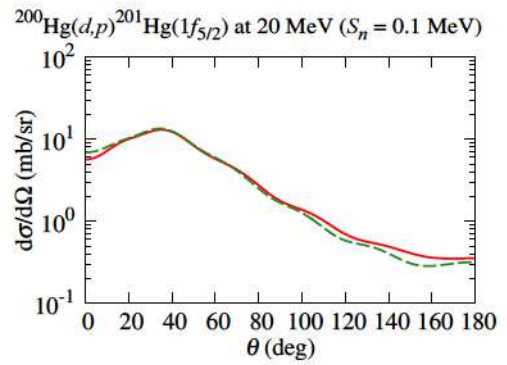



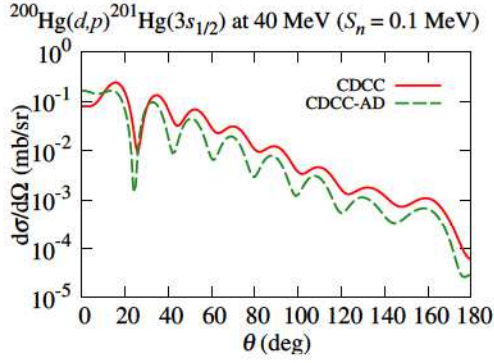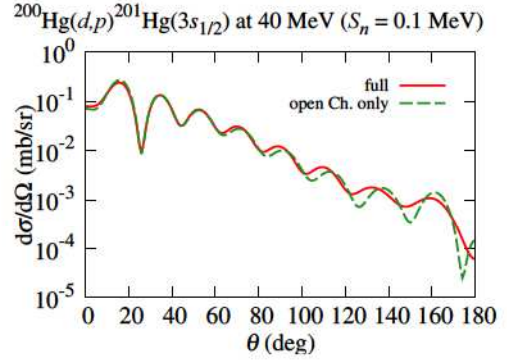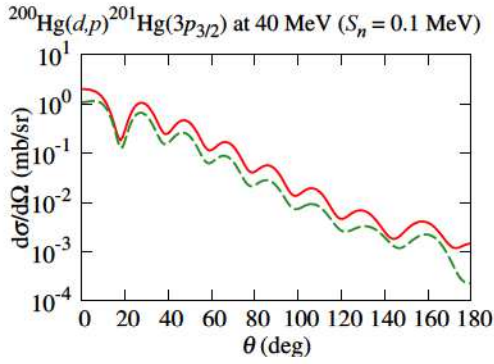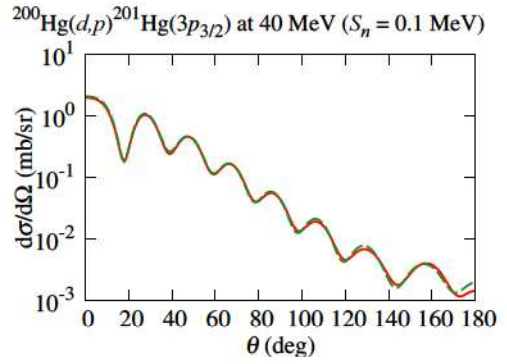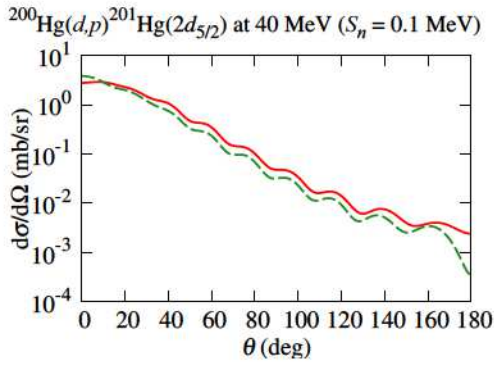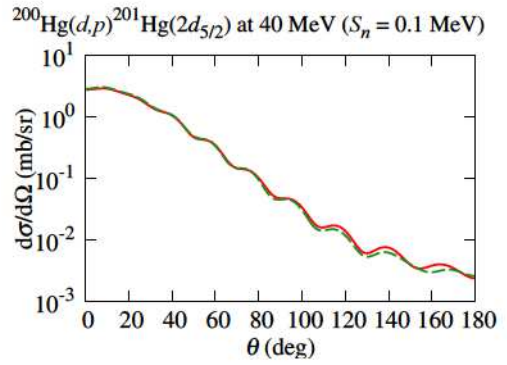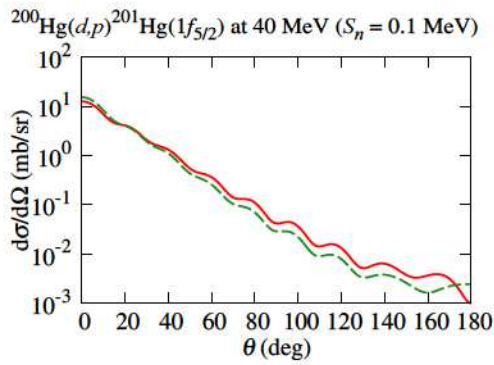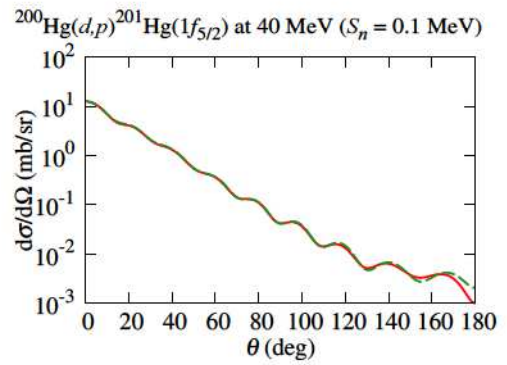

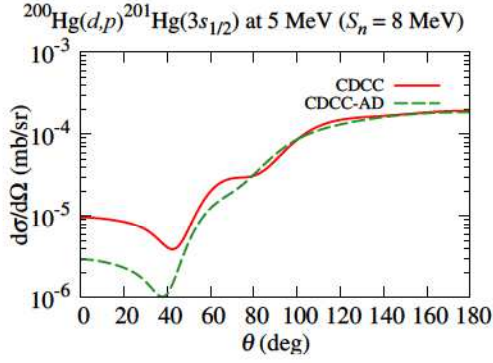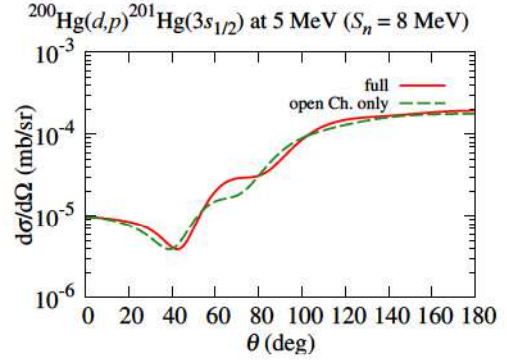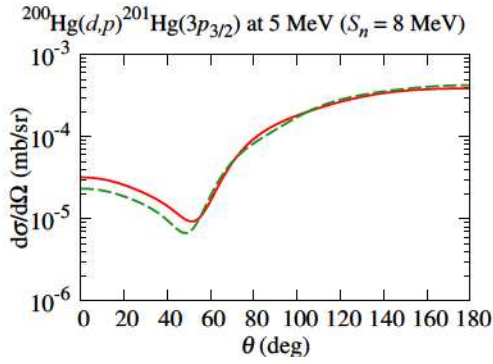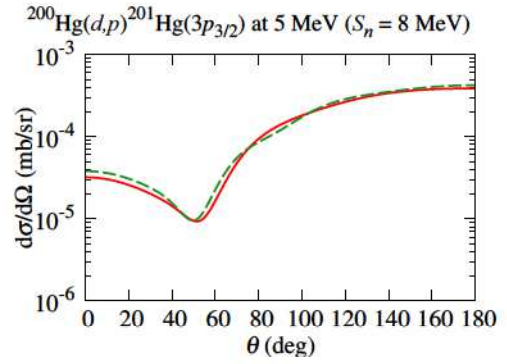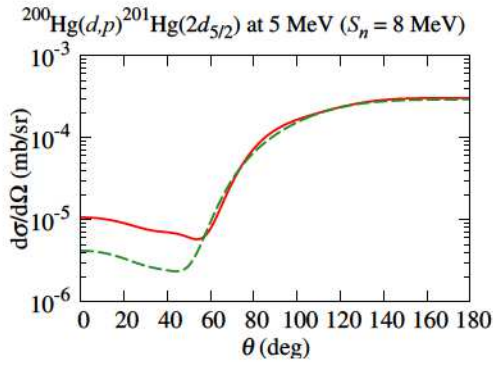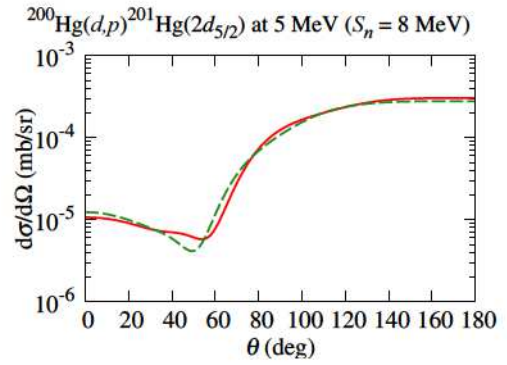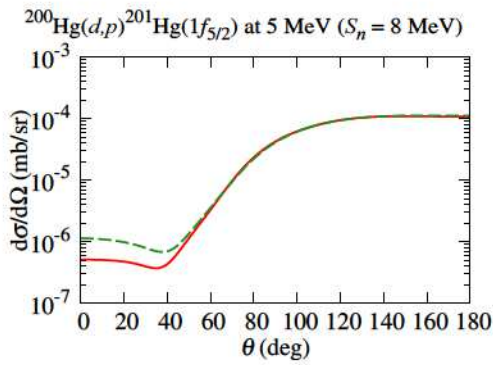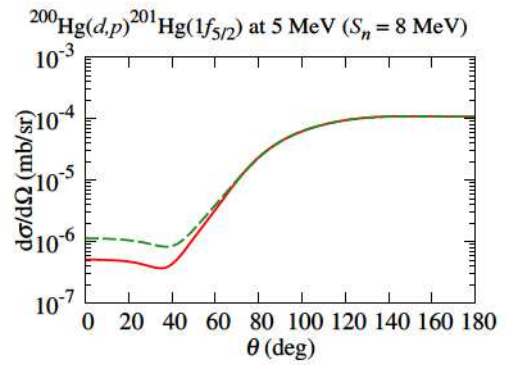

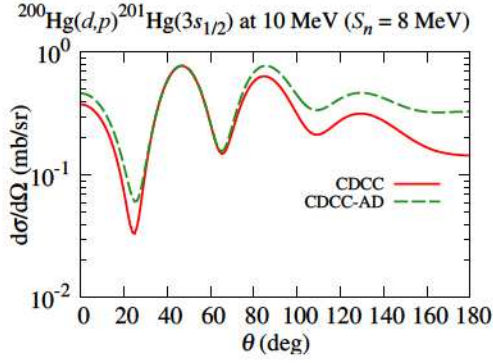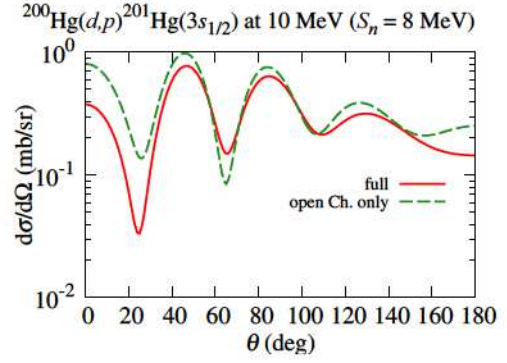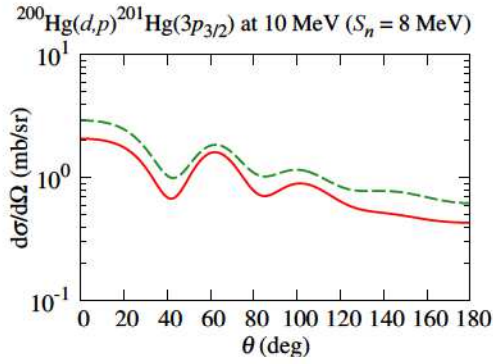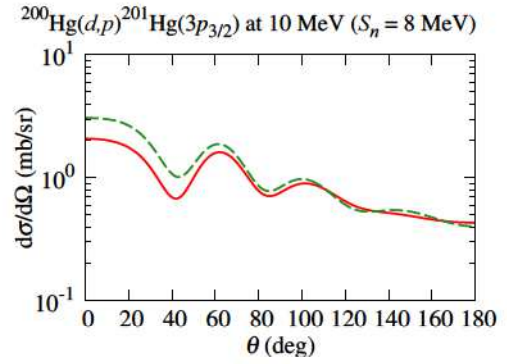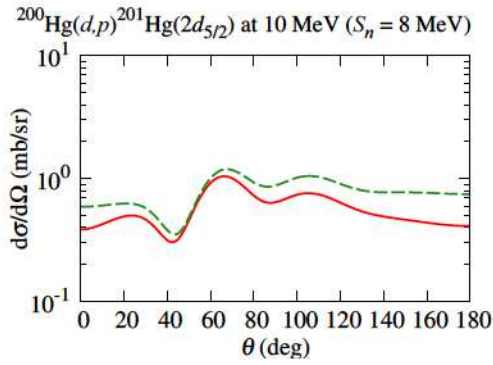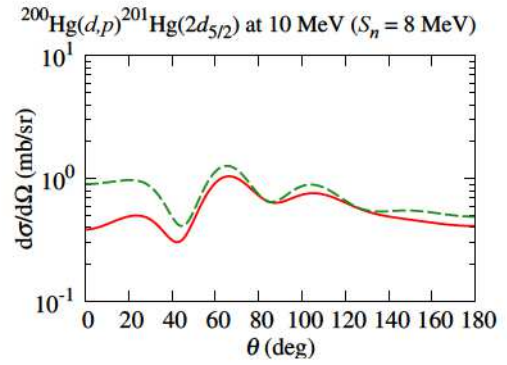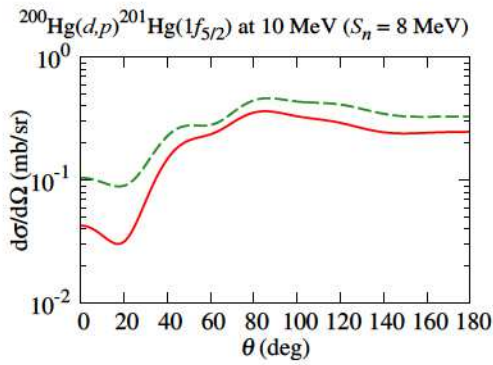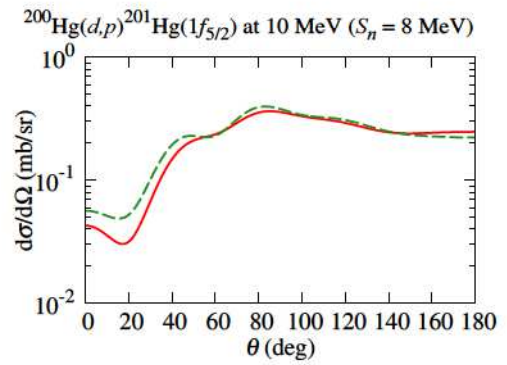

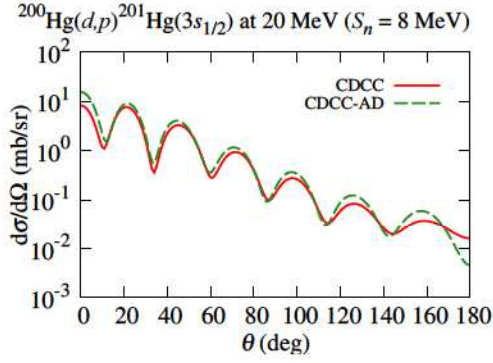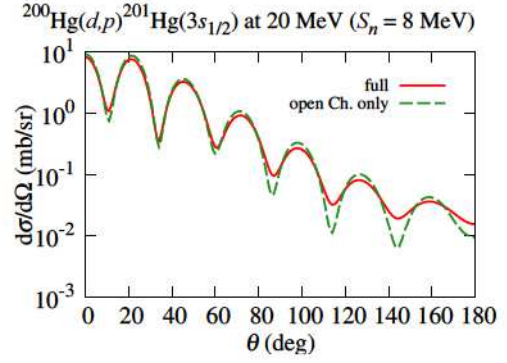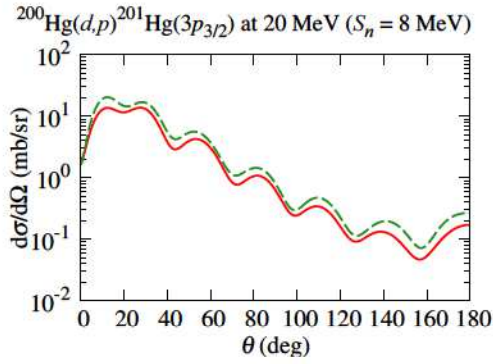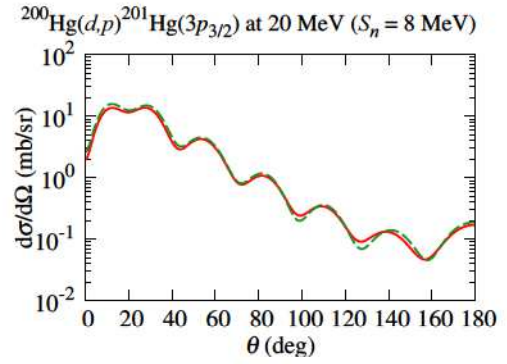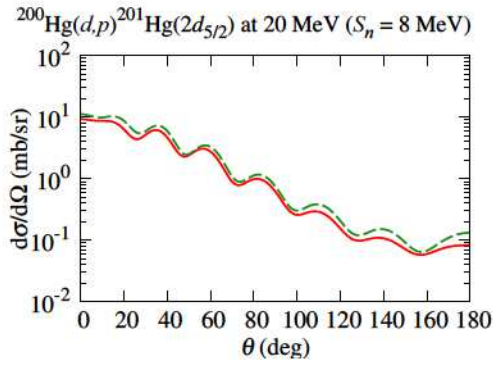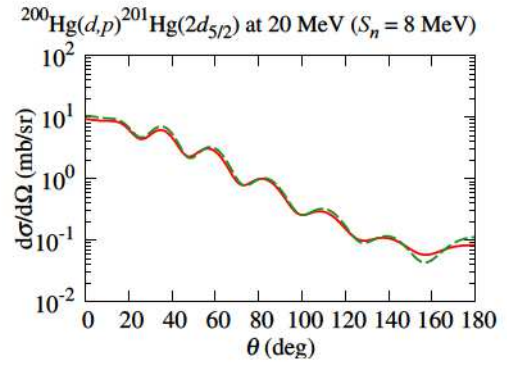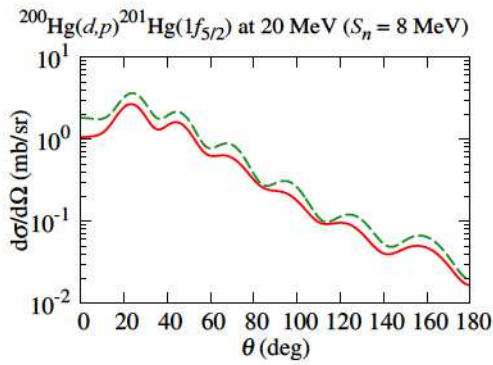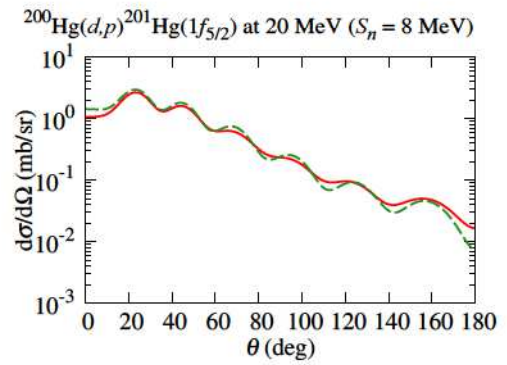



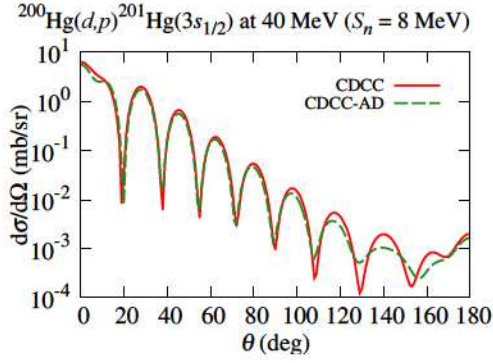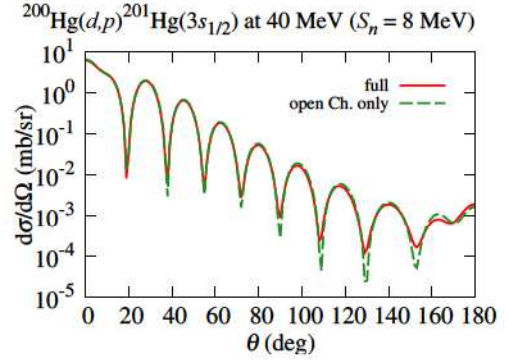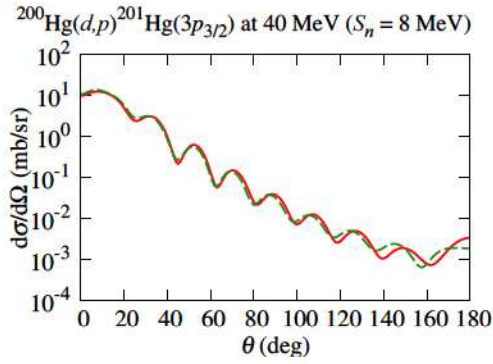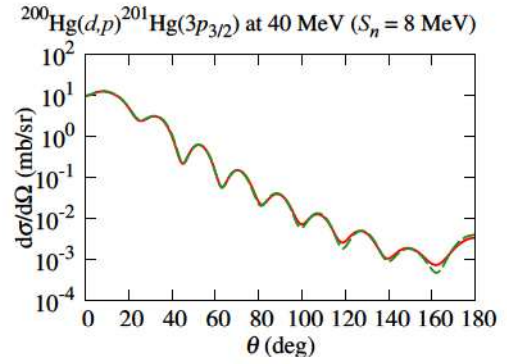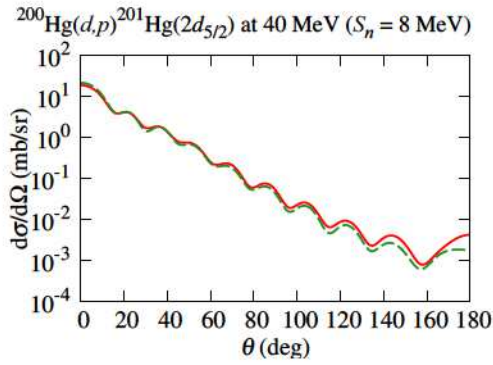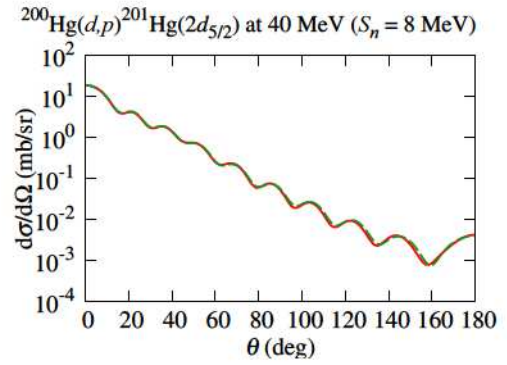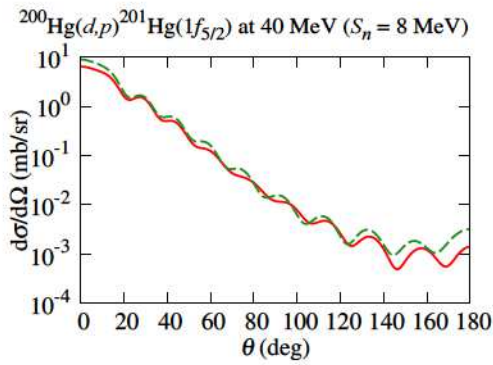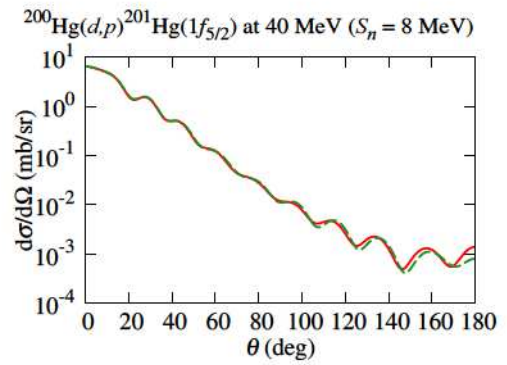

Supplement: Supplementary file 1 [file addendum_for_arXiv.pdf]
